# Supplementary material for: The EBLM Project XI. Mass, radius and effective temperature measurements for 23 M-dwarf companions to solar-type stars observed with CHEOPS
Source: arXiv:2312.11339 ancillary file (2023-12-18)
Supplement: Supplementary file 1 [file EBLMXI_AppendixTables.pdf]

**Table 1.** The derived parameters for the targets EBLM J0057-19, EBLM J0113+31, EBLM J0123+38, EBLM J0239-20, EBLM J0540-17 and EBLM J0546-18; calculated by our `PYCHEOPS` fits of *CHEOPS* and *TESS* light curves. We also present the spectroscopic surface gravity ($\log g_{1,sp.}$) and microturbulence velocity $v_{mic}$ calculated by the *CHEOPS* TS3 team.

| | J0057-19 | J0113+31 | J0123+38 | J0239-20 | J0540-17 | J0546-18 |
|---|---|---|---|---|---|---|
| Spectr. params | | | | | | |
| $\log g_{1,sp.}$ (cgs) | 4.27 ± 0.10 | 4.10 ± 0.11 | 4.30 ± 0.14 | 4.08 ± 0.20 | 3.955 ± 0.120 | 4.0 ± 0.8 |
| $v_{mic}$ (kms$^{-1}$) | 1 ± 0 | 1.07 ± 0.06 | 1.67 ± 0.10 | 1 ± 0 | 1.191 ± 0.060 | −− |
| CHEOPS Model params | | | | | | |
| $T_0$ (BJD) | 1767.3843 ± 0.0002 | 2335.4973 ± 0.0001 | 2164.3360 ± 0.0002 | 2163.7080 ± 0.0001 | 2209.1209 ± 0.0002 | 2203.7145 ± 0.0003 |
| $P$ (days) | = 4.30055 | = 14.27684 | = 7.95294 | = 2.77869 | = 6.00494 | = 3.19190 |
| $D$ | 0.0195 ± 0.0004 | 0.0228 ± 0.0001 | 0.0300 ± 0.0002 | 0.0168 ± 0.0002 | 0.0140 ± 0.0002 | 0.0239 ± 0.0019 |
| $W$ | 0.0365 ± 0.0002 | 0.0190 ± 0.0001 | 0.0387 ± 0.0003 | 0.0527 ± 0.0004 | 0.0382 ± 0.0002 | 0.0415 ± 0.0016 |
| $b$ | 0.368 ± 0.063 | 0.320 ± 0.009 | 0.186 ± 0.095 | 0.654 ± 0.014 | 0.167 ± 0.105 | 0.777 ± 0.041 |
| $f_c$ | = 0.0 | 0.0871 ± 0.0002$^\dagger$ | = 0.0 | = 0.0 | = 0.0 | = 0.0 |
| $f_s$ | = 0.0 | −0.5489 ± 0.0004$^\dagger$ | = 0.0 | = 0.0 | = 0.0 | = 0.0 |
| $L$ | 0.00042 ± 0.00012 | 0.00083 ± 0.00005 | 0.00102 ± 0.00008 | 0.00037 ± 0.00005 | 0.00037 ± 0.00005 | 0.00111 ± 0.00013 |
| $h_1$ | 0.800 ± 0.020 | 0.769 ± 0.004 | 0.818 ± 0.009 | 0.767 ± 0.020 | 0.767 ± 0.015 | 0.440 ± 0.144 |
| $h_2$ | 0.502 ± 0.230 | 0.667 ± 0.093 | 0.622 ± 0.169 | 0.469 ± 0.219 | 0.54 ± 0.18 | 0.308 ± 0.137 |
| Derived params | | | | | | |
| $R_2/R_1$ | 0.1395 ± 0.0014 | 0.1509 ± 0.0003 | 0.1733 ± 0.0007 | 0.1296 ± 0.0007 | 0.1185 ± 0.0009 | 0.1547 ± 0.0062 |
| $R_1/a$ | 0.1064 ± 0.0024 | 0.0539 ± 0.0003 | 0.1049 ± 0.0020 | 0.1797 ± 0.0003 | 0.1084 ± 0.0018 | 0.1534 ± 0.0060 |
| $R_2/a$ | 0.0143 ± 0.0004 | 0.0081 ± 0.0001 | 0.0178 ± 0.0004 | 0.0229 ± 0.0004 | 0.0127 ± 0.0003 | 0.0223 ± 0.0015 |
| $i$ (°) | 87.75 ± 0.43 | 89.01 ± 0.03 | 88.88 ± 0.59 | 83.25 ± 0.24 | 88.96 ± 0.67 | 83.16 ± 0.56 |
| $e$ | 0.0 | 0.3089 ± 0.0004 | 0.0 | 0.0 | 0.0 | 0.0 |
| $\omega$ (°) | −− | −80.98 ± 0.03 | −− | −− | −− | −− |
| Absolute params | | | | | | |
| $M_2$ ($M_\odot$) | 0.1290 ± 0.0052 | 0.1974 ± 0.0068 | 0.338 ± 0.012 | 0.1598 ± 0.0059 | 0.1633 ± 0.0058 | 0.2129 ± 0.0075 |
| $R_2$ ($R_\odot$) | 0.1722 ± 0.0054 | 0.2161 ± 0.0041 | 0.3498 ± 0.0097 | 0.2056 ± 0.0053 | 0.1939 ± 0.0050 | 0.2330 ± 0.0130 |
| $\log g_1$ (cgs) | 4.257 ± 0.022 | 4.141 ± 0.010 | 3.894 ± 0.019 | 4.053 ± 0.016 | 4.058 ± 0.017 | 4.099 ± 0.035 |
| $\log g_2$ (cgs) | 5.076 ± 0.021 | 5.064 ± 0.005 | 4.883 ± 0.017 | 5.015 ± 0.014 | 5.075 ± 0.015 | 5.028 ± 0.048 |
| $T_{eff,2}$ (K) | 2958 ± 124 | 3258 ± 37 | 3404 ± 71 | 3027 ± 58 | 3220 ± 70 | 3412 ± 80 |
| TESS Model params | | | | | | |
| $T_0$ (BJD) | 1338.9354 ± 0.0002 | 1778.7003 ± 0.0002 | 1776.6884 ± 0.0005 | 1413.4614 ± 0.0001 | 1470.5128 ± 0.0003 | 2174.9866 ± 0.0003 |
| $P$ (days) | 4.30055 ± 0.00001 | 14.28099 ± 0.00322 | 7.95267 ± 0.00034 | 2.77869 ± 0.00001 | 6.00494 ± 0.00001 | 3.19192 ± 0.00003 |
| $D$ | 0.0185 ± 0.0002 | 0.0239 ± 0.0002 | 0.0300 ± 0.0005 | 0.0166 ± 0.0001 | 0.0138 ± 0.0002 | 0.0233 ± 0.0008 |
| $W$ | 0.0365 ± 0.0002 | 0.0191 ± 0.0001 | 0.0394 ± 0.0002 | 0.0527 ± 0.0001 | 0.0383 ± 0.0002 | 0.0402 ± 0.0005 |
| $b$ | 0.376 ± 0.039 | 0.338 ± 0.017 | 0.188 ± 0.101 | 0.644 ± 0.009 | 0.254 ± 0.089 | 0.824 ± 0.013 |
| $f_c$ | = 0.0 | 0.0869 ± 0.0002$^\dagger$ | = 0.0 | = 0.0 | = 0.0 | = 0.0 |
| $f_s$ | = 0.0 | −0.5489 ± 0.0004$^\dagger$ | = 0.0 | = 0.0 | = 0.0 | = 0.0 |
| $L$ | 0.00054 ± 0.00008 | 0.00160 ± 0.00008 | 0.00261 ± 0.00013 | 0.00077 ± 0.00004 | 0.00066 ± 0.00008 | 0.00176 ± 0.00012 |
| $h_1$ | 0.829 ± 0.013 | 0.820 ± 0.012 | 0.782 ± 0.018 | 0.841 ± 0.011 | 0.811 ± 0.013 | 0.717 ± 0.101 |
| $h_2$ | 0.383 ± 0.278 | 0.517 ± 0.226 | 0.521 ± 0.205 | 0.598 ± 0.193 | 0.466 ± 0.205 | 0.355 ± 0.244 |
| Derived params | | | | | | |
| $R_2/R_1$ | 0.1361 ± 0.0009 | 0.1546 ± 0.0008 | 0.1733 ± 0.0015 | 0.1288 ± 0.0003 | 0.1175 ± 0.0007 | 0.1526 ± 0.0028 |
| $R_1/a$ | 0.1069 ± 0.0017 | 0.0545 ± 0.0006 | 0.1069 ± 0.0017 | 0.1787 ± 0.0014 | 0.1105 ± 0.0023 | 0.1568 ± 0.0027 |
| $R_2/a$ | 0.0143 ± 0.0003 | 0.0083 ± 0.0001 | 0.0182 ± 0.0004 | 0.0228 ± 0.0002 | 0.0126 ± 0.0003 | 0.0236 ± 0.0003 |
| $i$ (°) | 87.69 ± 0.28 | 88.94 ± 0.06 | 88.85 ± 0.64 | 83.39 ± 0.14 | 88.39 ± 0.60 | 82.58 ± 0.23 |
| $e$ | 0.0 | 0.3088 ± 0.0004 | 0.0 | 0.0 | 0.0 | 0.0 |
| $\omega$ (°) | −− | −81.00 ± 0.02 | −− | −− | −− | −− |
| Absolute params | | | | | | |
| $M_2$ ($M_\odot$) | 0.1289 ± 0.0052 | 0.1975 ± 0.0068 | 0.338 ± 0.012 | 0.1597 ± 0.0059 | 0.1633 ± 0.0057 | 0.2132 ± 0.0075 |
| $R_2$ ($R_\odot$) | 0.1689 ± 0.0045 | 0.2236 ± 0.0049 | 0.3566 ± 0.0094 | 0.2032 ± 0.0043 | 0.1959 ± 0.0056 | 0.2356 ± 0.0074 |
| $\log g_1$ (cgs) | 4.252 ± 0.017 | 4.132 ± 0.013 | 3.877 ± 0.017 | 4.057 ± 0.011 | 4.042 ± 0.020 | 4.080 ± 0.018 |
| $\log g_2$ (cgs) | 5.093 ± 0.015 | 5.035 ± 0.010 | 4.866 ± 0.016 | 5.025 ± 0.007 | 5.066 ± 0.019 | 5.021 ± 0.022 |
| $T_{eff,2}$ (K) | 2750 ± 77 | 3227 ± 38 | 3544 ± 63 | 3014 ± 41 | 3142 ± 66 | 3331 ± 56 |

$^\dagger$: Derived parameters based on Gaussian priors from spectroscopic or radial velocity data.

**Table 2.** The derived parameters for the *CHEOPS* targets EBLM J0719+25, EBLM J0941-31, EBLM J0955-39, EBLM J1013+01, EBLM J1305-31 and EBLM J1522+42; calculated by our PYCHEOPS fits of *CHEOPS* and *TESS* light curves. We also present the spectroscopic surface gravity (log $g_{1,sp.}$) and microturbulence velocity $v_{mic}$ calculated by the *CHEOPS* TS3 team.

| | J0719+25 | J0941-31 | J0955-39 | J1013+01 | J1305-31 | J1522+42 |
|---|---|---|---|---|---|---|
| Spectr. parameters | | | | | | |
| $\log g_{1,spectr.}$ (cgs) | 4.35 ± 0.11 | 3.948 ± 0.191 | 4.5 ± 0.8 | 3.56 ± 0.80 | 4.083 ± 0.109 | 4.23 ± 0.11 |
| $v_{mic}$ (kms$^{-1}$) | 1.12 ± 0.04 | 1.701 ± 0.108 | −− | −− | 1.154 ± 0.031 | 0.885 ± 0.028 |
| CHEOPS<br>Model params | | | | | | |
| $T_0$ (BJD) | 2216.3900 ± 0.0002 | 2278.9545 ± 0.0002 | 2290.7348 ± 0.0006 | 2244.3407 ± 0.0002 | 2311.3193 ± 0.0002 | = 2317.3518 |
| $P$ (days) | = 7.45629 | = 5.54563 | = 5.31360 | = 2.89227 | = 10.61913 | = 7.66134 |
| $D$ | 0.0213 ± 0.0003 | 0.0180 ± 0.0003 | 0.0450 ± 0.0008 | 0.0432 ± 0.0007 | 0.0405 ± 0.0006 | = 0.0197 |
| $W$ | 0.0250 ± 0.0003 | 0.0407 ± 0.0001 | 0.0270 ± 0.0003 | 0.0431 ± 0.0002 | 0.0206 ± 0.0001 | = 0.0285 |
| $b$ | 0.502 ± 0.031 | 0.343 ± 0.062 | 0.489 ± 0.034 | 0.082 ± 0.065 | 0.704 ± 0.012 | = 0.148 |
| $f_c$ | −0.2589 ± 0.0068† | 0.4436 ± 0.0012† | = 0.0 | = 0.0 | −0.1725 ± 0.0014† | −0.2184 ± 0.0053† |
| $f_s$ | −0.1163 ± 0.0228† | 0.0390 ± 0.0040† | = 0.0 | = 0.0 | −0.0859 ± 0.0024† | −0.2767 ± 0.0137† |
| $L$ | 0.00064 ± 0.00012 | 0.00063 ± 0.00007 | 0.00153 ± 0.00026 | 0.00162 ± 0.00016 | 0.00104 ± 0.00014 | 0.00053 ± 0.00011 |
| $h_1$ | 0.749 ± 0.009† | 0.829 ± 0.017 | 0.808 ± 0.034 | 0.710 ± 0.017 | 0.785 ± 0.056 | −− |
| $h_2$ | 0.408 ± 0.051† | 0.598 ± 0.193 | 0.397 ± 0.273 | 0.384 ± 0.192 | 0.344 ± 0.281 | −− |
| Derived params | | | | | | |
| $R_2/R_1$ | 0.1460 ± 0.0010 | 0.1341 ± 0.0010 | 0.2121 ± 0.0019 | 0.2079 ± 0.0017 | 0.2013 ± 0.0016 | −− |
| $R_1/a$ | 0.0763 ± 0.0018 | 0.1183 ± 0.0021 | 0.0764 ± 0.0015 | 0.1124 ± 0.0009 | 0.0665 ± 0.0008 | −− |
| $R_2/a$ | 0.0108 ± 0.0003 | 0.0155 ± 0.0004 | 0.0158 ± 0.0004 | 0.0232 ± 0.0002 | 0.0133 ± 0.0001 | −− |
| $i$ (°) | 87.81 ± 0.19 | 87.67 ± 0.46 | 87.86 ± 0.18 | 89.47 ± 0.42 | 87.32 ± 0.07 | −− |
| $e$ | 0.0808 ± 0.0041 | 0.1984 ± 0.0010 | 0.0 | 0.0 | 0.0371 ± 0.0006 | −− |
| $\omega$ (°) | −155.80 ± 4.57 | 5.03 ± 0.52 | −− | −− | −153.53 ± 0.69 | −− |
| Absolute params | | | | | | |
| $M_2$ ($M_\odot$) | 0.1584 ± 0.0055 | 0.2173 ± 0.0078 | 0.2211 ± 0.0080 | 0.1706 ± 0.0062 | 0.2820 ± 0.0095 | −− |
| $R_2$ ($R_\odot$) | 0.1919 ± 0.0057 | 0.2340 ± 0.0064 | 0.2325 ± 0.0060 | 0.2093 ± 0.0045 | 0.3007 ± 0.0072 | −− |
| $\log g_1$ (cgs) | 4.233 ± 0.022 | 4.027 ± 0.018 | 4.432 ± 0.019 | 4.424 ± 0.011 | 4.116 ± 0.014 | = 4.168 ± 0.014 |
| $\log g_2$ (cgs) | 5.071 ± 0.021 | 5.037 ± 0.017 | 5.048 ± 0.019 | 5.029 ± 0.010 | 4.932 ± 0.013 | = 5.093 ± 0.013 |
| $T_{eff,2}$ (K) | 3212 ± 89 | 3448 ± 72 | 3332 ± 90 | 3043 ± 49 | 3135 ± 64 | 3064 ± 86 |
| TESS<br>Model params | | | | | | |
| $T_0$ (BJD) | 2559.3826 ± 0.0002 | 1519.2002 ± 0.0001 | 1546.8317 ± 0.0002 | 1518.3782 ± 0.0001 | 1578.5980 ± 0.0003 | 1934.2851 ± 0.0002 |
| $P$ (days) | 7.45629 ± 0.00005 | 5.54565 ± 0.00001 | 5.31359 ± 0.00001 | 2.89228 ± 0.00001 | 10.61914 ± 0.00001 | 7.66134 ± 0.00001 |
| $D$ | 0.0209 ± 0.0002 | 0.0179 ± 0.0001 | 0.0459 ± 0.0004 | 0.0417 ± 0.0002 | 0.0420 ± 0.0004 | 0.0197 ± 0.0002 |
| $W$ | 0.0250 ± 0.0002 | 0.0410 ± 0.0001 | 0.0269 ± 0.0001 | 0.0425 ± 0.0001 | 0.0205 ± 0.0001 | 0.0285 ± 0.0002 |
| $b$ | 0.520 ± 0.016 | 0.382 ± 0.022 | 0.471 ± 0.016 | 0.106 ± 0.046 | 0.672 ± 0.012 | 0.148 ± 0.075 |
| $f_c$ | −0.2588 ± 0.0054† | 0.4440 ± 0.0005† | = 0.0 | = 0.0 | −0.1742 ± 0.0011† | −0.2205 ± 0.0042† |
| $f_s$ | −0.1385 ± 0.0225† | 0.0389 ± 0.0039† | = 0.0 | = 0.0 | −0.0868 ± 0.0024† | −0.2751 ± 0.0115† |
| $L$ | 0.00093 ± 0.00006 | 0.00121 ± 0.00005 | 0.00284 ± 0.00015 | 0.00292 ± 0.00004 | 0.00104 ± 0.00014 | 0.00112 ± 0.00006 |
| $h_1$ | 0.812 ± 0.013 | 0.826 ± 0.007 | 0.828 ± 0.016 | 0.795 ± 0.004 | 0.836 ± 0.038 | 0.768 ± 0.009 |
| $h_2$ | 0.553 ± 0.195 | 0.558 ± 0.184 | 0.492 ± 0.206 | = 0.420 | 0.505 ± 0.203 | 0.584 ± 0.150 |
| Derived params | | | | | | |
| $R_2/R_1$ | 0.1446 ± 0.0006 | 0.1338 ± 0.0004 | 0.2141 ± 0.0010 | 0.2041 ± 0.0004 | 0.2050 ± 0.0009 | 0.1404 ± 0.0007 |
| $R_1/a$ | 0.0769 ± 0.0010 | 0.1206 ± 0.0010 | 0.0756 ± 0.0006 | 0.1114 ± 0.0004 | 0.0644 ± 0.0006 | 0.0792 ± 0.0010 |
| $R_2/a$ | 0.0110 ± 0.0002 | 0.0160 ± 0.0002 | 0.0160 ± 0.0002 | 0.0226 ± 0.0001 | 0.0130 ± 0.0002 | 0.0110 ± 0.0002 |
| $i$ (°) | 87.71 ± 0.10 | 87.36 ± 0.18 | 87.96 ± 0.09 | 89.32 ± 0.29 | 87.52 ± 0.06 | 89.33 ± 0.346 |
| $e$ | 0.0862 ± 0.0036 | 0.1987 ± 0.0004 | 0.0 | 0.0 | 0.0379 ± 0.0005 | 0.1243 ± 0.0045 |
| $\omega$ (°) | −151.86 ± 4.35 | 5.00 ± 0.51 | −− | −− | −153.53 ± 0.67 | −128.70 ± 1.70 |
| Absolute params | | | | | | |
| $M_2$ ($M_\odot$) | 0.1583 ± 0.0055 | 0.2173 ± 0.0078 | 0.2220 ± 0.0079 | 0.1712 ± 0.0062 | 0.2820 ± 0.0094 | 0.1657 ± 0.0063 |
| $R_2$ ($R_\odot$) | 0.1917 ± 0.0044 | 0.2380 ± 0.0050 | 0.2327 ± 0.0048 | 0.2042 ± 0.0039 | 0.2963 ± 0.0063 | 0.1915 ± 0.0043 |
| $\log g_1$ (cgs) | 4.225 ± 0.014 | 4.010 ± 0.012 | 4.442 ± 0.012 | 4.433 ± 0.010 | 4.144 ± 0.012 | 4.168 ± 0.014 |
| $\log g_2$ (cgs) | 5.072 ± 0.012 | 5.022 ± 0.008 | 5.049 ± 0.008 | 5.052 ± 0.004 | 4.945 ± 0.009 | 5.093 ± 0.013 |
| $T_{eff,2}$ (K) | 3063 ± 40 | 3421 ± 47 | 3285 ± 41 | 3017 ± 30 | 3174 ± 44 | 3073 ± 36 |

†: Derived parameters based on Gaussian priors from spectroscopic or radial velocity data.

**Table 3.** The derived parameters for the *CHEOPS* targets EBLM J1559-05, EBLM J1741+31, EBLM J1928-38, EBLM J1934-42, EBLM J2040-41 and EBLM J2046-40; calculated by our PYCHEOPS fits of *CHEOPS* and *TESS* light curves. We also present the spectroscopic surface gravity (log $g_{1,sp.}$) and microturbulence velocity $v_{mic}$ calculated by the *CHEOPS* TS3 team.

| | J1559-05 | J1741+31 | J1928-38 | J1934-42 | J2040-41 | J2046-40 |
|---|---|---|---|---|---|---|
| Spectr. params | | | | | | |
| $\log g_{1,\mathrm{spectr.}}$ (cgs) | $4.37 \pm 0.10$ | $4.63 \pm 0.11$ | $4.015 \pm 0.102$ | $4.327 \pm 0.119$ | $4.084 \pm 0.103$ | $4.009 \pm 0.117$ |
| $v_{mic}$ (kms$^{-1}$) | −− | $1.25 \pm 0.05$ | $1.079 \pm 0.021$ | $1.099 \pm 0.042$ | $1.005 \pm 0.035$ | $0.983 \pm 0.059$ |
| CHEOPS Model params | | | | | | |
| $T_0$ (BJD) | $2347.2225 \pm 0.0001$ | $2014.0489 \pm 0.0001$ | $2375.4273 \pm 0.0002$ | $2028.2295 \pm 0.0002$ | $2433.8913 \pm 0.0005$ | $= 2604.942$ |
| $P$ (days) | $= 3.76008$ | $= 7.71262$ | $= 23.32286$ | $= 6.35251$ | $= 14.45626$ | $= 37.0143$ |
| $D$ | $0.0139 \pm 0.0005$ | $0.1446 \pm 0.0445$ | $0.0378 \pm 0.0004$ | $0.0540 \pm 0.0122$ | $0.0177 \pm 0.0003$ | $= 0.0316$ |
| $W$ | $0.0429 \pm 0.0002$ | $0.0104 \pm 0.0027$ | $0.0134 \pm 0.0001$ | $0.0191 \pm 0.0003$ | $0.0184 \pm 0.0003$ | $= 0.0092$ |
| $b$ | $0.701 \pm 0.007$ | $1.274 \pm 0.116$ | $0.395 \pm 0.019$ | $0.812 \pm 0.053$ | $0.176 \pm 0.118$ | $= 0.152$ |
| $f_c$ | $= 0.0$ | $0.3003 \pm 0.0016^\dagger$ | $-0.1989 \pm 0.0006^\dagger$ | $= 0.0$ | $0.3810 \pm 0.0005^\dagger$ | $-0.6279 \pm 0.0002^\dagger$ |
| $f_s$ | $= 0.0$ | $0.4592 \pm 0.0012^\dagger$ | $-0.1840 \pm 0.0007^\dagger$ | $= 0.0$ | $-0.2852 \pm 0.0007^\dagger$ | $0.2826 \pm 0.0006^\dagger$ |
| $L$ | $0.00029 \pm 0.00002$ | −− | $0.00126 \pm 0.00008$ | $0.00133 \pm 0.00043$ | $0.00032 \pm 0.00007$ | $0.00087 \pm 0.00007$ |
| $h_1$ | $0.660 \pm 0.075$ | $0.765 \pm 0.011^\dagger$ | $0.732 \pm 0.009$ | $0.730 \pm 0.011^\dagger$ | $0.733 \pm 0.015$ | −− |
| $h_2$ | $0.080 \pm 0.085$ | $0.429 \pm 0.050^\dagger$ | $0.553 \pm 0.149$ | $0.396 \pm 0.050^\dagger$ | $0.305 \pm 0.197$ | −− |
| Derived params | | | | | | |
| $R_2/R_1$ | $0.1177 \pm 0.0022$ | $0.380 \pm 0.057$ | $0.1945 \pm 0.0010$ | $0.2323 \pm 0.0247$ | $0.1329 \pm 0.0013$ | −− |
| $R_1/a$ | $0.1547 \pm 0.0015$ | $0.0610 \pm 0.0006$ | $0.0373 \pm 0.0003$ | $0.0646 \pm 0.0018$ | $0.0517 \pm 0.0016$ | −− |
| $R_2/a$ | $0.0179 \pm 0.0004$ | $0.0203 \pm 0.0035$ | $0.0072 \pm 0.0001$ | $0.0141 \pm 0.0021$ | $0.0067 \pm 0.0002$ | −− |
| $i$ (°) | $83.78 \pm 0.12$ | $85.53 \pm 0.42$ | $89.16 \pm 0.05$ | $86.99 \pm 0.29$ | $89.48 \pm 0.37$ | −− |
| $e$ | 0.0 | $0.3009 \pm 0.0015$ | $0.0734 \pm 0.0004$ | 0.0 | $0.2265 \pm 0.0005$ | −− |
| $\omega$ (°) | −− | $56.81 \pm 0.16$ | $-137.24 \pm 0.15$ | −− | $-36.82 \pm 0.07$ | −− |
| Absolute params | | | | | | |
| $M_2$ ($M_\odot$) | $0.1568 \pm 0.0058$ | $0.461 \pm 0.015$ | $0.2703 \pm 0.0091$ | $0.1960 \pm 0.0076$ | $0.1524 \pm 0.0053$ | −− |
| $R_2$ ($R_\odot$) | $0.2011 \pm 0.0058$ | $0.450 \pm 0.068$ | $0.2692 \pm 0.0057$ | $0.239 \pm 0.026$ | $0.1797 \pm 0.0065$ | −− |
| $\log g_1$ (cgs) | $4.024 \pm 0.012$ | $4.367 \pm 0.013$ | $4.153 \pm 0.012$ | $4.471 \pm 0.027$ | $4.174 \pm 0.028$ | $= 4.273 \pm 0.011$ |
| $\log g_2$ (cgs) | $5.025 \pm 0.019$ | $4.790 \pm 0.130$ | $5.010 \pm 0.009$ | $4.997 \pm 0.096$ | $5.111 \pm 0.028$ | $= 5.032 \pm 0.008$ |
| $T_{\mathrm{eff},2}$ (K) | $3139 \pm 50$ | −− | $3153 \pm 36$ | $3014 \pm 98$ | $2910 \pm 89$ | $3127 \pm 43$ |
| TESS Model parameters | | | | | | |
| $T_0$ (BJD) | −− | $1990.9112 \pm 0.0001$ | −− | $1659.7838 \pm 0.0002$ | $2043.5742 \pm 0.0006$ | $1346.4552 \pm 0.0003$ |
| $P$ (days) | −− | $7.71264 \pm 0.00001$ | −− | $6.35251 \pm 0.00001$ | $14.45534 \pm 0.00083$ | $37.01362 \pm 0.00002$ |
| $D$ | −− | $0.0986 \pm 0.0020$ | −− | $0.0476 \pm 0.0011$ | $0.0176 \pm 0.0002$ | $0.0316 \pm 0.0003$ |
| $W$ | −− | $0.0127 \pm 0.0002$ | −− | $0.0190 \pm 0.0001$ | $0.0187 \pm 0.0001$ | $0.0092 \pm 0.0001$ |
| $b$ | −− | $1.141 \pm 0.011$ | −− | $0.787 \pm 0.009$ | $0.124 \pm 0.090$ | $0.152 \pm 0.111$ |
| $f_c$ | −− | $0.3005 \pm 0.0020^\dagger$ | −− | $= 0.0$ | $0.3812 \pm 0.0005^\dagger$ | $-0.6276 \pm 0.0003^\dagger$ |
| $f_s$ | −− | $0.4589 \pm 0.0016^\dagger$ | −− | $= 0.0$ | $-0.2853 \pm 0.0007^\dagger$ | $0.2825 \pm 0.0006^\dagger$ |
| $L$ | −− | −− | −− | $0.00212 \pm 0.00028$ | $0.00089 \pm 0.00016$ | $0.00194 \pm 0.00015$ |
| $h_1$ | −− | $0.807 \pm 0.012^\dagger$ | −− | $0.786 \pm 0.011^\dagger$ | $0.780 \pm 0.018$ | $0.764 \pm 0.013$ |
| $h_2$ | −− | $0.412 \pm 0.057^\dagger$ | −− | $0.389 \pm 0.050^\dagger$ | $0.428 \pm 0.196$ | $0.518 \pm 0.179$ |
| Derived params | | | | | | |
| $R_2/R_1$ | −− | $0.3140 \pm 0.0032$ | −− | $0.2182 \pm 0.0024$ | $0.1325 \pm 0.0009$ | $0.1778 \pm 0.0010$ |
| $R_1/a$ | −− | $0.0612 \pm 0.0003$ | −− | $0.0641 \pm 0.0007$ | $0.0521 \pm 0.0008$ | $0.0247 \pm 0.0002$ |
| $R_2/a$ | −− | $0.0189 \pm 0.0002$ | −− | $0.0137 \pm 0.0003$ | $0.0068 \pm 0.0001$ | $0.0044 \pm 0.0001$ |
| $i$ (°) | −− | $86.00 \pm 0.05$ | −− | $87.11 \pm 0.06$ | $89.63 \pm 0.27$ | $89.78 \pm 0.16$ |
| $e$ | −− | $0.3007 \pm 0.0019$ | −− | 0.0 | $0.2267 \pm 0.0005$ | $0.4737 \pm 0.0004$ |
| $\omega$ (°) | −− | $56.79 \pm 0.20$ | −− | −− | $-36.81 \pm 0.08$ | $155.77 \pm 0.05$ |
| Absolute params | | | | | | |
| $M_2$ ($M_\odot$) | −− | $0.460 \pm 0.015$ | −− | $0.1967 \pm 0.0070$ | $0.1524 \pm 0.0053$ | $0.1917 \pm 0.0067$ |
| $R_2$ ($R_\odot$) | −− | $0.3729 \pm 0.0083$ | −− | $0.2229 \pm 0.0051$ | $0.1804 \pm 0.0044$ | $0.2212 \pm 0.0046$ |
| $\log g_1$ (cgs) | −− | $4.365 \pm 0.011$ | −− | $4.478 \pm 0.013$ | $4.168 \pm 0.016$ | $4.273 \pm 0.011$ |
| $\log g_2$ (cgs) | −− | $4.958 \pm 0.010$ | −− | $5.038 \pm 0.014$ | $5.108 \pm 0.014$ | $5.032 \pm 0.008$ |
| $T_{\mathrm{eff},2}$ (K) | −− | −− | −− | $2959 \pm 64$ | $3014 \pm 90$ | $3163 \pm 50$ |

$^\dagger$: Derived parameters based on Gaussian priors from spectroscopic or radial velocity data.

**Table 4.** The derived parameters for the *CHEOPS* targets EBLM J2046+06, EBLM J2134+19, EBLM J2315+23, EBLM J2343+29 and EBLM J2359+44; calculated by our `PYCHEOPS` fits of *CHEOPS* and *TESS* light curves. We also present the spectroscopic surface gravity (log $g_{1,\rm sp.}$) and microturbulence velocity $v_{\rm mic}$ calculated by the *CHEOPS* TS3 team.

| | J2046+06 | J2134+19 | J2315+23 | J2343+29 | J2359+44 |
|---|---|---|---|---|---|
| Spectr. parameters | | | | | |
| $\log g_{1,\rm spectr.}$ (cgs) | 3.984 ± 0.105 | 4.00 ± 0.11 | 4.26 ± 0.11 | 4.25 ± 0.18 | 4.68 ± 0.12 |
| $v_{\rm mic}$ (kms$^{-1}$) | 1.612 ± 0.048 | 0.76 ± 0.04 | 1.18 ± 0.04 | 0.42 ± 0.20 | 2.10 ± 0.09 |
| CHEOPS Model params | | | | | |
| $T_0$ (BJD) | 2090.6246 ± 0.0001 | 2462.2840 ± 0.0011 | 2476.1268 ± 0.0002 | 2458.6659 ± 0.0001 | 1977.9726 ± 0.0001 |
| $P$ (days) | = 10.10779 | 16.58571 ± 0.00005 | = 9.13105 | = 16.95353 | = 11.35602 |
| $D$ | 0.0162 ± 0.0002 | 0.0410 ± 0.0003 | 0.0269 ± 0.0003 | 0.0256 ± 0.0003 | 0.0300 ± 0.0002 |
| $W$ | 0.0261 ± 0.0002 | 0.0201 ± 0.0002 | 0.0279 ± 0.0002 | 0.01070 ± 0.00005 | 0.0260 ± 0.0001 |
| $b$ | 0.254 ± 0.050 | 0.645 ± 0.013 | 0.190 ± 0.092 | 0.290 ± 0.038 | 0.0970 ± 0.0239 |
| $f_c$ | −0.1904 ± 0.0006$^\dagger$ | 0.4360 ± 0.0061$^\dagger$ | −0.3241 ± 0.0009$^\dagger$ | 0.0806 ± 0.0006$^\dagger$ | −0.0532 ± 0.0003$^\dagger$ |
| $f_s$ | 0.5545 ± 0.0004$^\dagger$ | 0.2706 ± 0.0214$^\dagger$ | −0.2088 ± 0.0020$^\dagger$ | 0.3924 ± 0.0004$^\dagger$ | −0.6890 ± 0.0007$^\dagger$ |
| $L$ | 0.00033 ± 0.00002 | 0.00388 ± 0.00013 | 0.00097 ± 0.00011 | 0.00031 ± 0.00005 | 0.00089 ± 0.00006 |
| $h_1$ | 0.761 ± 0.011 | 0.746 ± 0.009 | 0.816 ± 0.0103 | 0.697 ± 0.009 | 0.776 ± 0.004 |
| $h_2$ | 0.319 ± 0.161 | 0.598 ± 0.132 | 0.640 ± 0.157 | 0.377 ± 0.140 | 0.612 ± 0.131 |
| Derived params | | | | | |
| $R_2/R_1$ | 0.1274 ± 0.0007 | 0.2024 ± 0.0007 | 0.1641 ± 0.0009 | 0.1601 ± 0.0010 | 0.1731 ± 0.0005 |
| $R_1/a$ | 0.0747 ± 0.0005 | 0.0622 ± 0.0008 | 0.0765 ± 0.0015 | 0.0299 ± 0.0002 | 0.0698 ± 0.0003 |
| $R_2/a$ | 0.0094 ± 0.0001 | 0.0124 ± 0.0002 | 0.0123 ± 0.0003 | 0.0047 ± 0.0001 | 0.0120 ± 0.0001 |
| $i$ (°) | 88.91 ± 0.22 | 87.70 ± 0.07 | 89.17 ± 0.42 | 89.50 ± 0.07 | 89.61 ± 0.10 |
| $e$ | 0.3438 ± 0.0005 | 0.2633 ± 0.0064 | 0.1486 ± 0.0007 | 0.1604 ± 0.0003 | 0.4776 ± 0.0010 |
| $\omega$ (°) | 108.95 ± 0.05 | 31.84 ± 2.40 | −147.21 ± 0.29 | 78.39 ± 0.08 | −94.41 ± 0.03 |
| Absolute params | | | | | |
| $M_2$ ($M_\odot$) | 0.1769 ± 0.0062 | 0.359 ± 0.019 | 0.2309 ± 0.0099 | 0.1202 ± 0.0046 | 0.293 ± 0.010 |
| $R_2$ ($R_\odot$) | 0.2043 ± 0.0042 | 0.3706 ± 0.0088 | 0.2517 ± 0.0068 | 0.1464 ± 0.0029 | 0.2965 ± 0.0058 |
| $\log g_1$ (cgs) | 4.079 ± 0.011 | 3.860 ± 0.016 | 4.095 ± 0.019 | 4.596 ± 0.011 | 4.067 ± 0.010 |
| $\log g_2$ (cgs) | 5.065 ± 0.008 | 4.854 ± 0.019 | 5.000 ± 0.020 | 5.191 ± 0.008 | 4.960 ± 0.005 |
| $T_{\rm eff,2}$ (K) | 3124 ± 34 | 3496 ± 35 | 3298 ± 62 | 2572 ± 82 | 3462 ± 45 |
| TESS Model params | | | | | |
| $T_0$ (BJD) | 2090.6165 ± 0.0100 | = 2462.2840 | 2476.1443 ± 0.0156 | = 2458.6659 | 1773.4225 ± 0.0026 |
| $P$ (days) | 10.10771 ± 0.00014 | = 16.58558 | 9.13069 ± 0.00040 | = 16.95353 | 11.35338 ± 0.00264 |
| $D$ | 0.0160 ± 0.0001 | = 0.0410 | 0.0281 ± 0.0002 | = 0.0256 | 0.0302 ± 0.0002 |
| $W$ | 0.0259 ± 0.0002 | 0.0209 ± 0.0003 | 0.0278 ± 0.0001 | = 0.01070 | 0.0260 ± 0.0002 |
| $b$ | 0.353 ± 0.048 | = 0.645 | 0.058 ± 0.048 | = 0.290 | 0.120 ± 0.040 |
| $f_c$ | −0.1908 ± 0.0006$^\dagger$ | 0.4326 ± 0.0080$^\dagger$ | −0.3235 ± 0.0009$^\dagger$ | 0.0818 ± 0.0005$^\dagger$ | −0.0524 ± 0.0005$^\dagger$ |
| $f_s$ | 0.5546 ± 0.0004$^\dagger$ | 0.2805 ± 0.0277$^\dagger$ | −0.2084 ± 0.0019$^\dagger$ | 0.3925 ± 0.0004$^\dagger$ | −0.6890 ± 0.0007$^\dagger$ |
| $L$ | 0.00073 ± 0.00005 | 0.00700 ± 0.00011 | 0.00165 ± 0.00013 | 0.00071 ± 0.00005 | 0.00202 ± 0.00010 |
| $h_1$ | 0.811 ± 0.010 | −− | 0.824 ± 0.011 | −− | 0.824 ± 0.009 |
| $h_2$ | 0.595 ± 0.170 | −− | 0.557 ± 0.186 | −− | 0.565 ± 0.197 |
| Derived params | | | | | |
| $R_2/R_1$ | 0.1267 ± 0.0005 | −− | 0.1676 ± 0.0007 | −− | 0.1739 ± 0.0007 |
| $R_1/a$ | 0.0760 ± 0.0006 | −− | 0.0751 ± 0.0004 | −− | 0.0700 ± 0.0006 |
| $R_2/a$ | 0.0095 ± 0.0001 | −− | 0.0125 ± 0.0001 | −− | 0.0120 ± 0.0001 |
| $i$ (°) | 88.46 ± 0.22 | −− | 89.75 ± 0.21 | −− | 89.52 ± 0.16 |
| $e$ | 0.3439 ± 0.0005 | −− | 0.1480 ± 0.0007 | −− | 0.4775 ± 0.0010 |
| $\omega$ (°) | 108.98 ± 0.06 | −− | −147.20 ± 0.28 | −− | −94.35 ± 0.04 |
| Absolute params | | | | | |
| $M_2$ ($M_\odot$) | 0.1770 ± 0.0061 | −− | 0.2310 ± 0.0099 | −− | 0.293 ± 0.010 |
| $R_2$ ($R_\odot$) | 0.2067 ± 0.0042 | −− | 0.2523 ± 0.0059 | −− | 0.2989 ± 0.0064 |
| $\log g_1$ (cgs) | 4.064 ± 0.011 | = 3.860 ± 0.016 | 4.111 ± 0.010 | = 4.596 ± 0.011 | 4.064 ± 0.012 |
| $\log g_2$ (cgs) | 5.055 ± 0.008 | = 4.854 ± 0.019 | 4.998 ± 0.011 | = 5.191 ± 0.008 | 4.952 ± 0.000 |
| $T_{\rm eff,2}$ (K) | 3124 ± 42 | 3574 ± 42 | 3188 ± 47 | 2745 ± 36 | 3508 ± 42 |

$^\dagger$: Derived parameters based on Gaussian priors from spectroscopic or radial velocity data.
