# Supplementary material for: The EBLM Project XI. Mass, radius and effective temperature measurements for 23 M-dwarf companions to solar-type stars observed with CHEOPS
Source: arXiv:2312.11339 ancillary file (2023-12-18)
Supplement: Supplementary file 2 [file EBLMXI_AppendixPlots.pdf]

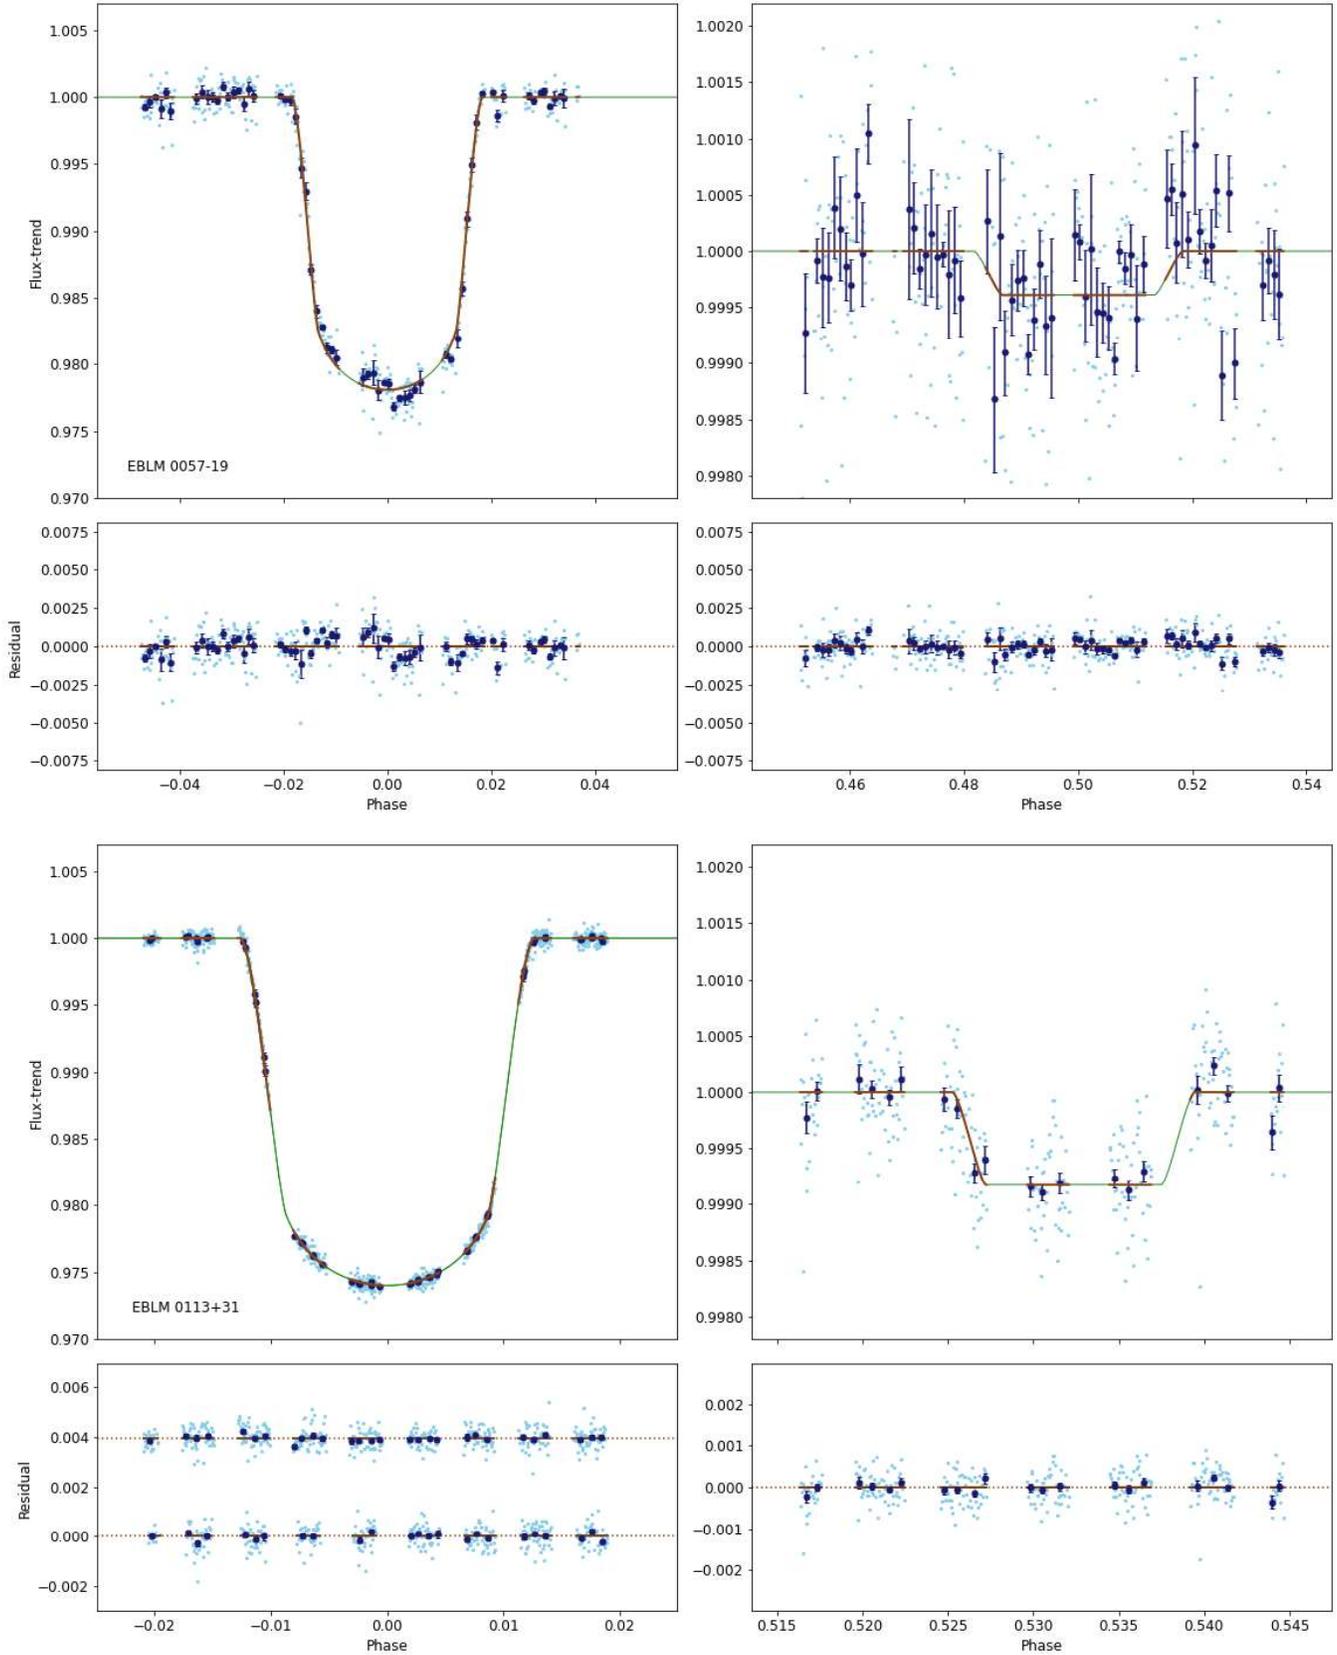

**Figure 1.** Fitted *CHEOPS* light curves of targets J0057-19 and J0113+31 in phase intervals around the primary and secondary eclipse events. The observed data points are shown in cyan. The transit and eclipse models are shown in green. Binned data points with error bars are shown in blue and the fit between binned data points in brown. The residual of the fit is displayed below the fitted curves.

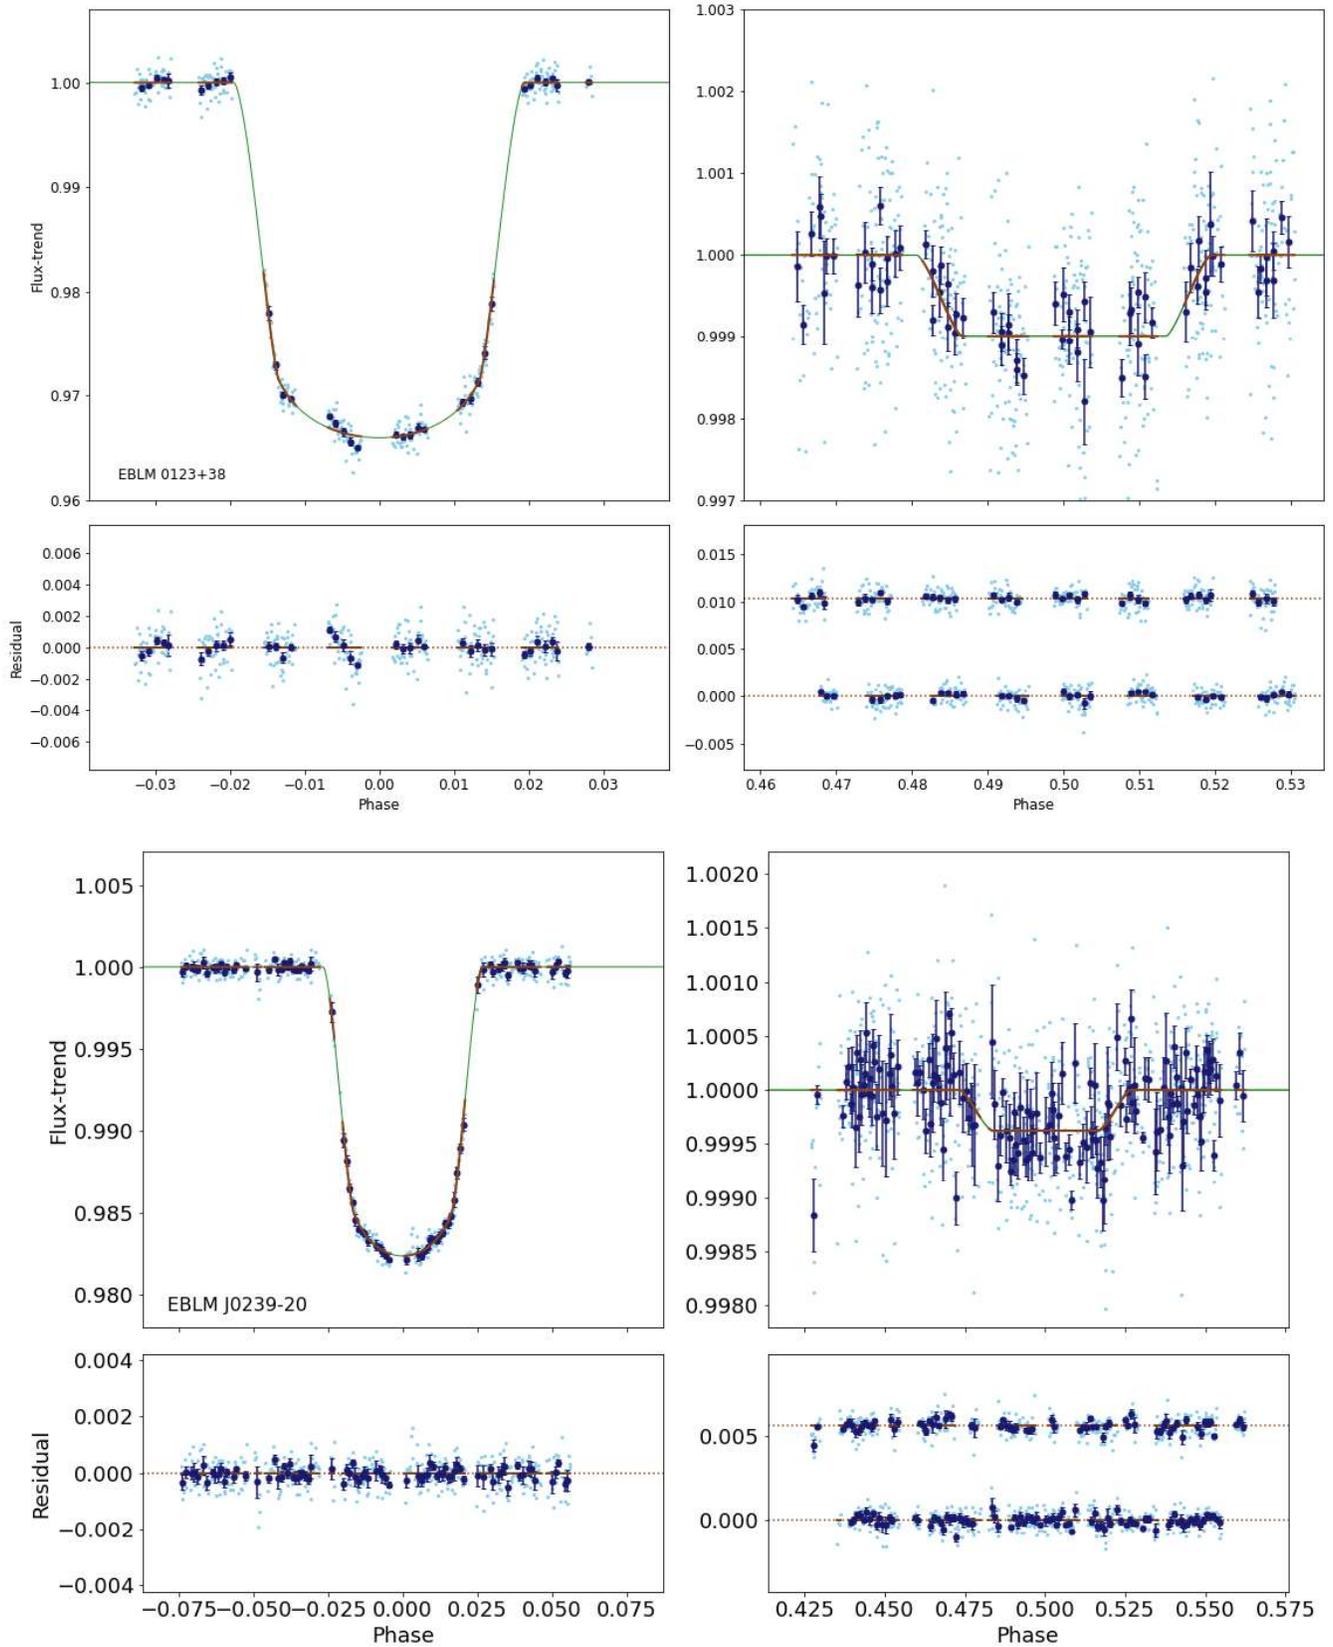

**Figure 2.** Fitted *CHEOPS* light curves of targets J0123+38 and J0239-20 in phase intervals around the primary and secondary eclipse events. The observed data points are shown in cyan. The transit and eclipse models are shown in green. Binned data points with error bars are shown in blue and the fit between binned data points in brown. The residual of the fit is displayed below the fitted curves.

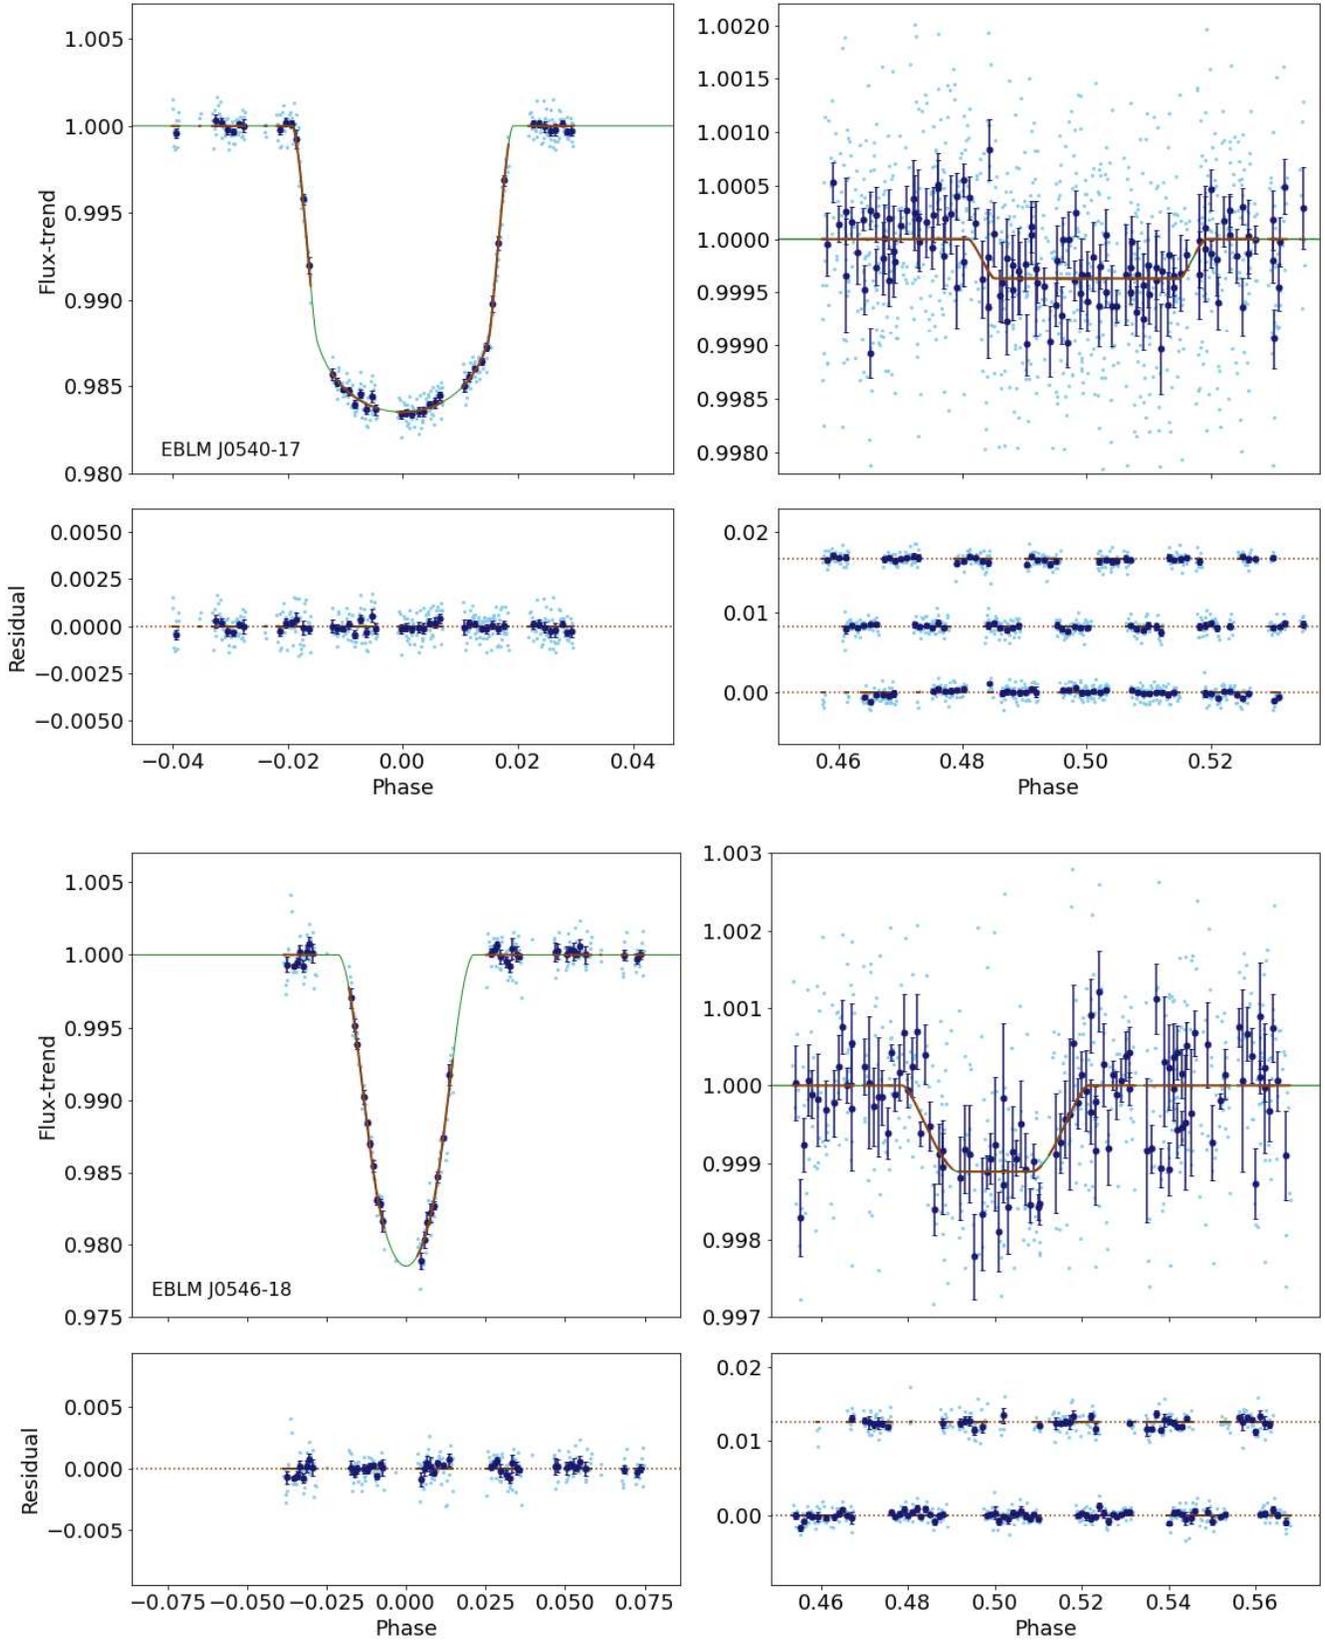

**Figure 3.** Fitted *CHEOPS* light curves of targets J0540-17 and J0546-18 in phase intervals around the primary and secondary eclipse events. The observed data points are shown in cyan. The transit and eclipse models are shown in green. Binned data points with error bars are shown in blue and the fit between binned data points in brown. The residual of the fit is displayed below the fitted curves.

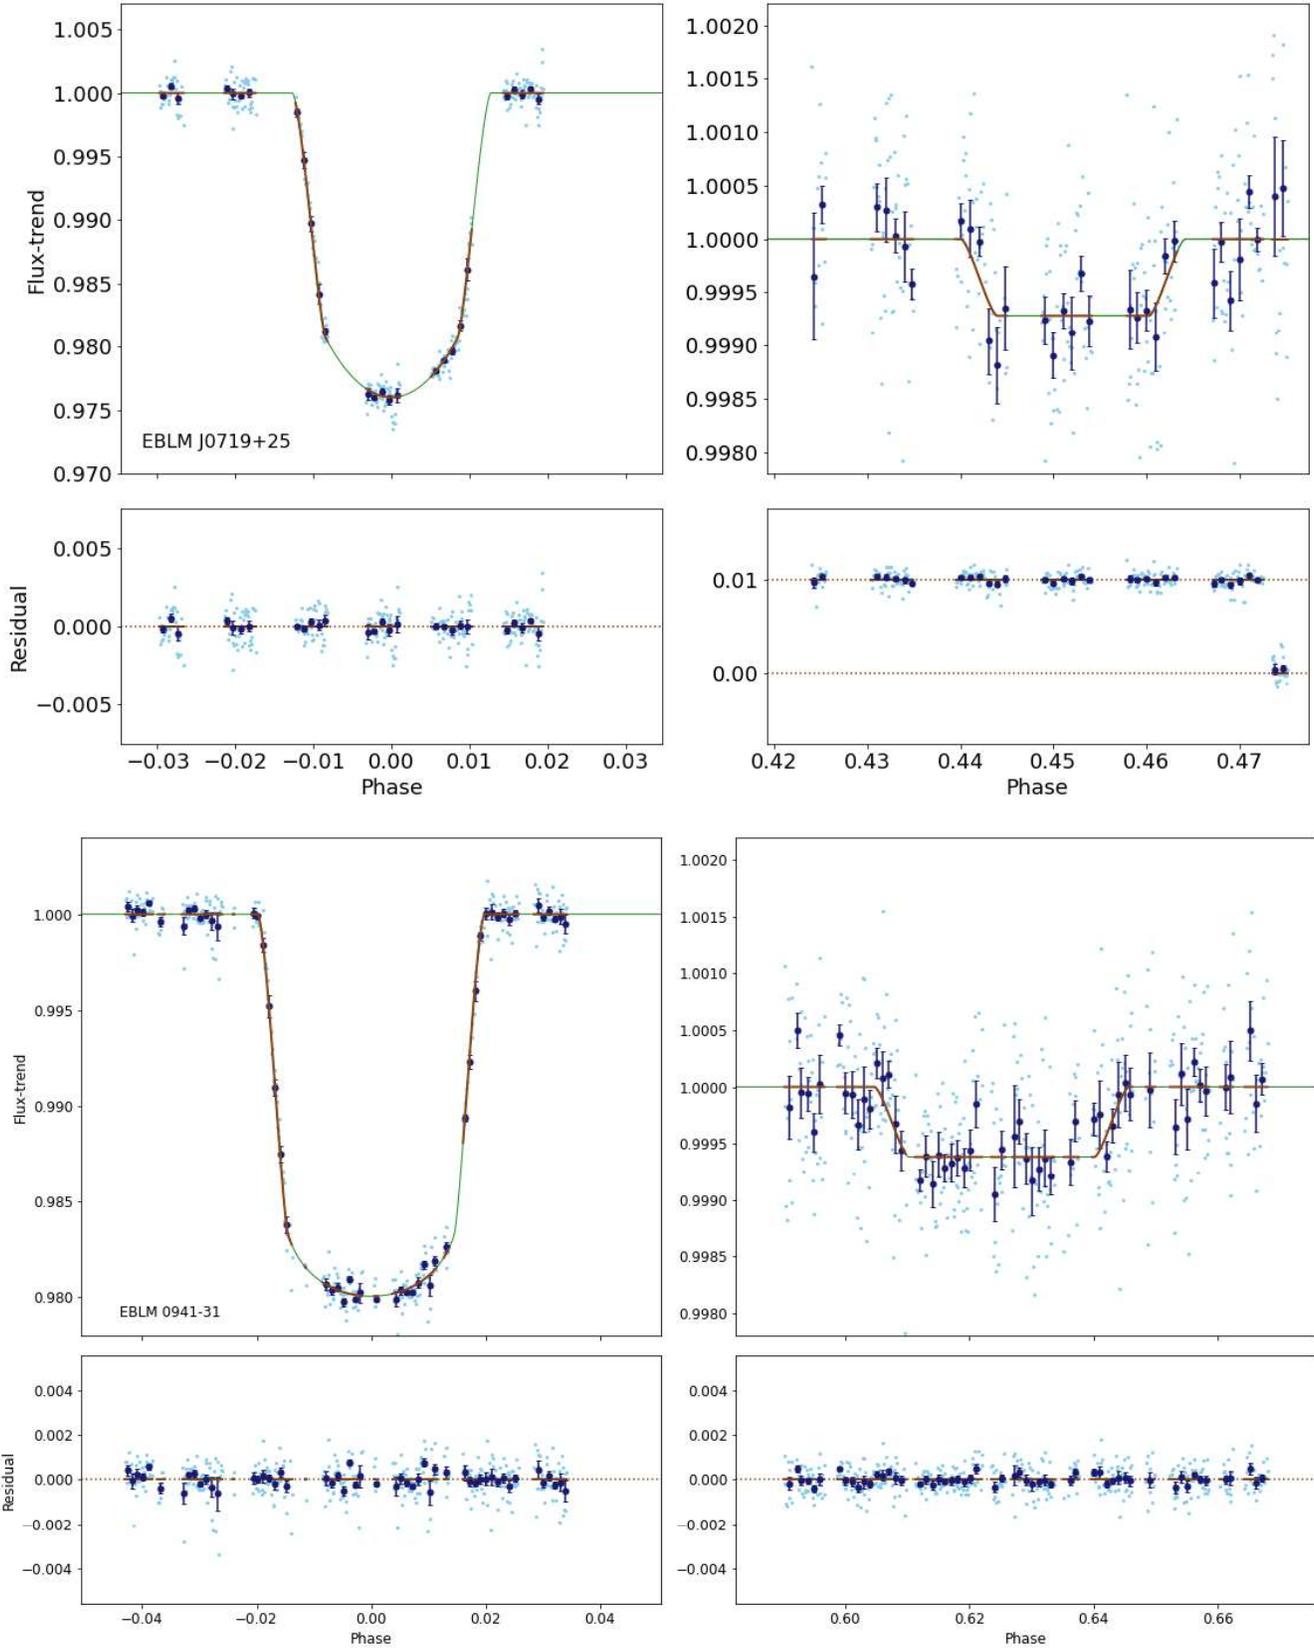

**Figure 4.** Fitted *CHEOPS* light curves of targets J0719+25 and J0941-31 in phase intervals around the primary and secondary eclipse events. The observed data points are shown in cyan. The transit and eclipse models are shown in green. Binned data points with error bars are shown in blue and the fit between binned data points in brown. The residual of the fit is displayed below the fitted curves.

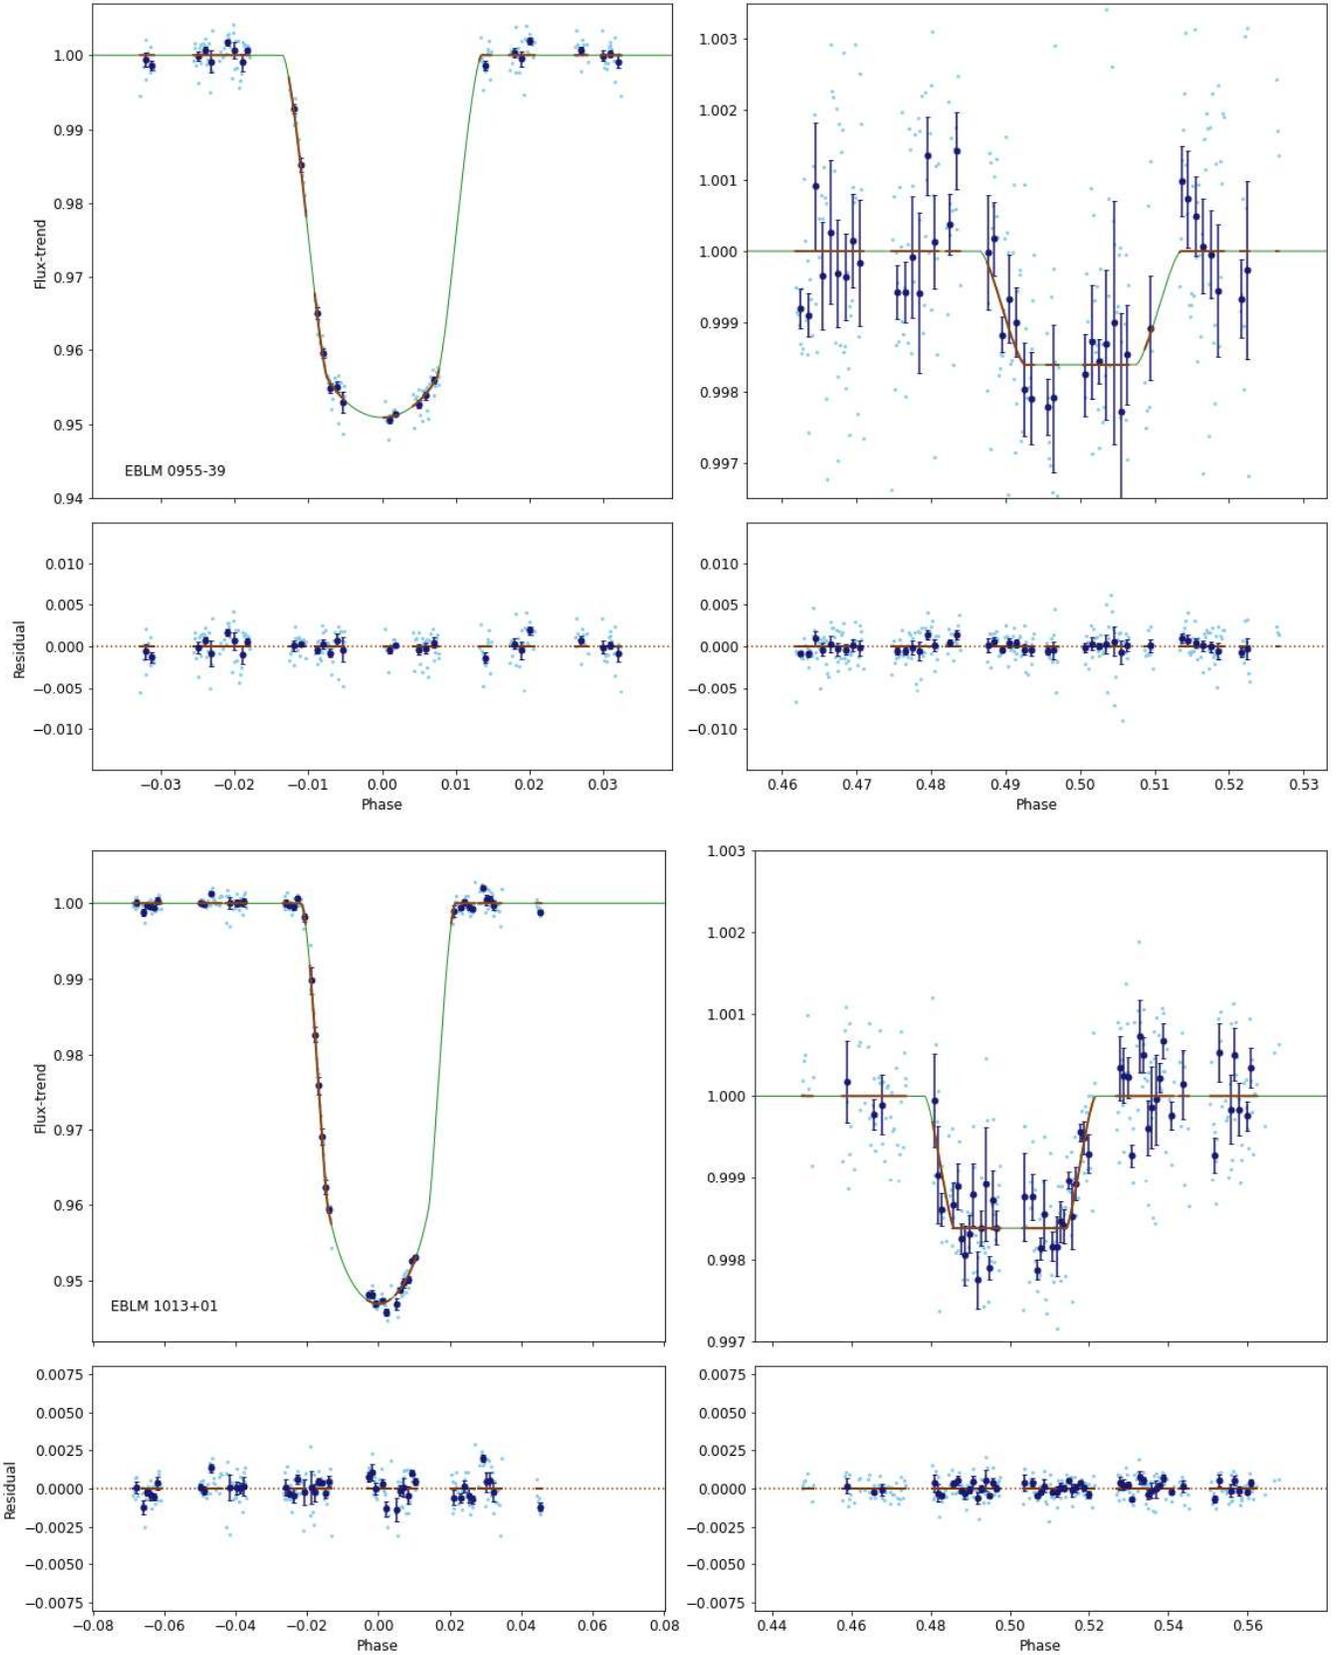

**Figure 5.** Fitted *CHEOPS* light curves of targets J0955-39 and J1013+01 in phase intervals around the primary and secondary eclipse events. The observed data points are shown in cyan. The transit and eclipse models are shown in green. Binned data points with error bars are shown in blue and the fit between binned data points in brown. The residual of the fit is displayed below the fitted curves.

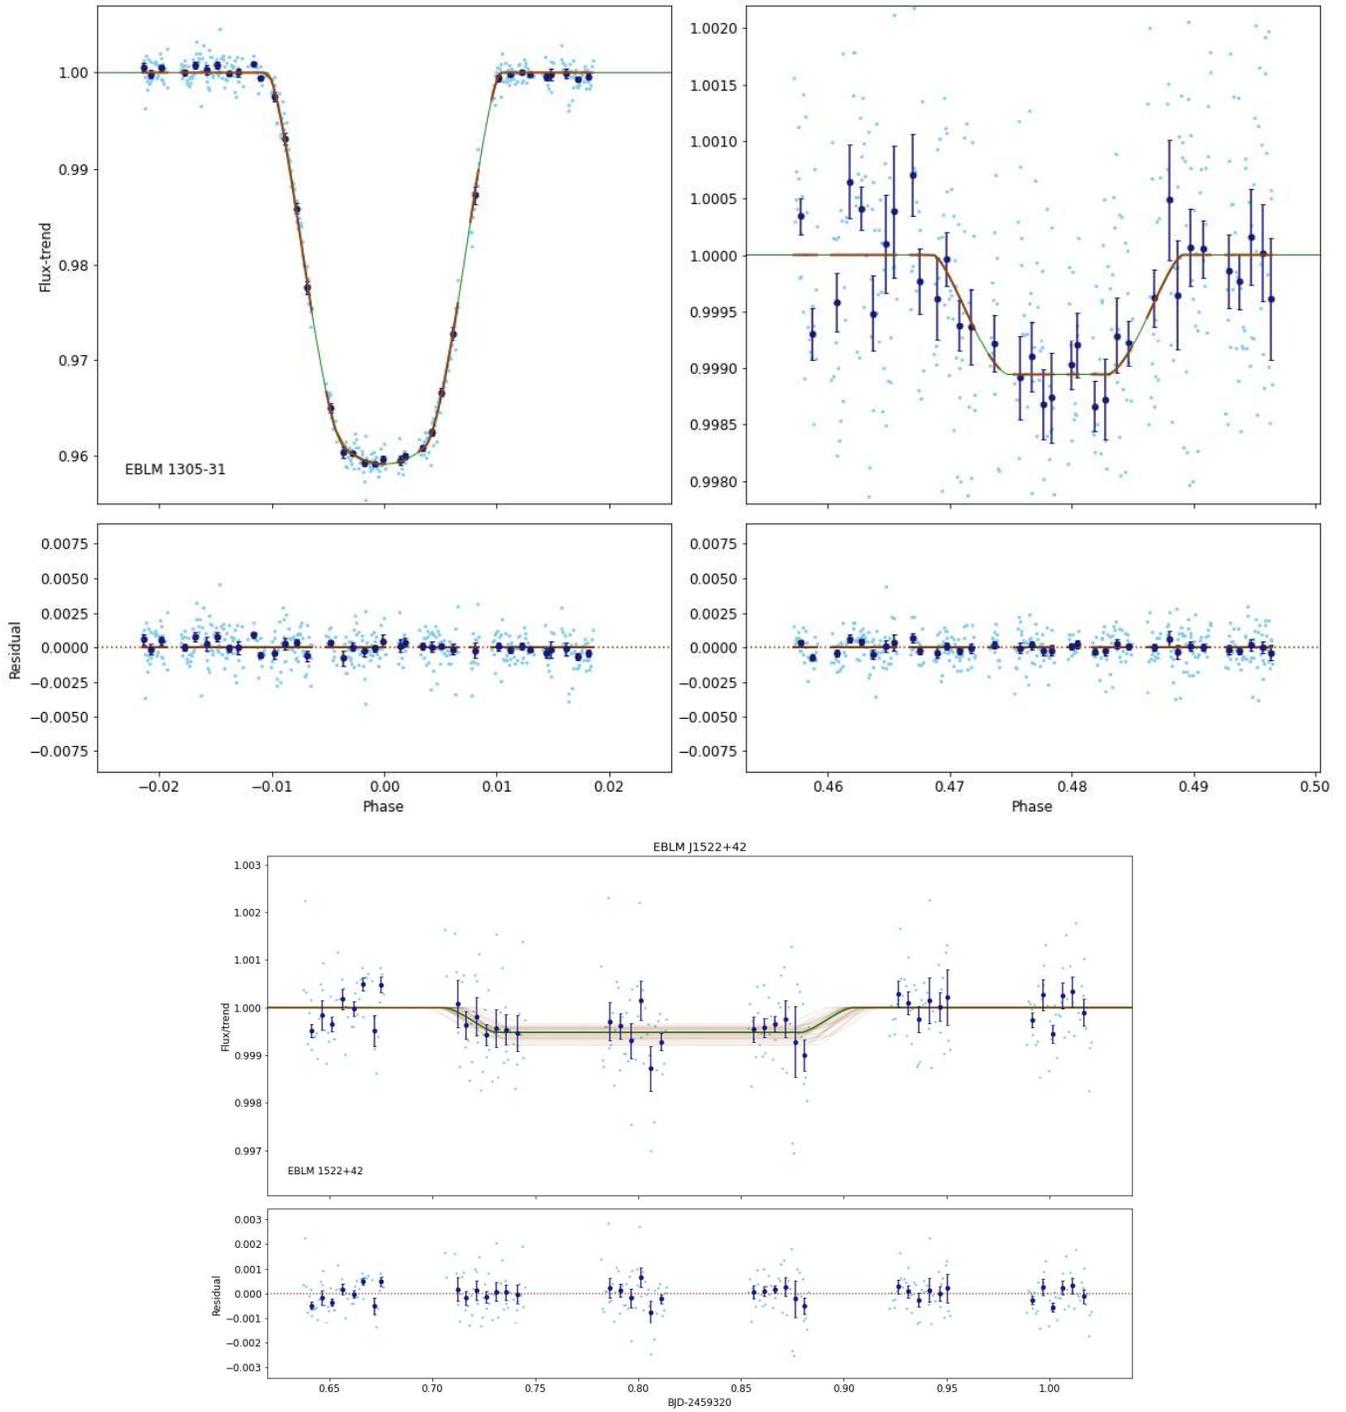

**Figure 6.** Fitted *CHEOPS* light curves of targets J1305-31 and J1522+42 in phase intervals around the primary and secondary eclipse events. The observed data points are shown in cyan. The transit and eclipse models are shown in green. Binned data points with error bars are shown in blue and the fit between binned data points in brown. The residual of the fit is displayed below the fitted curves.

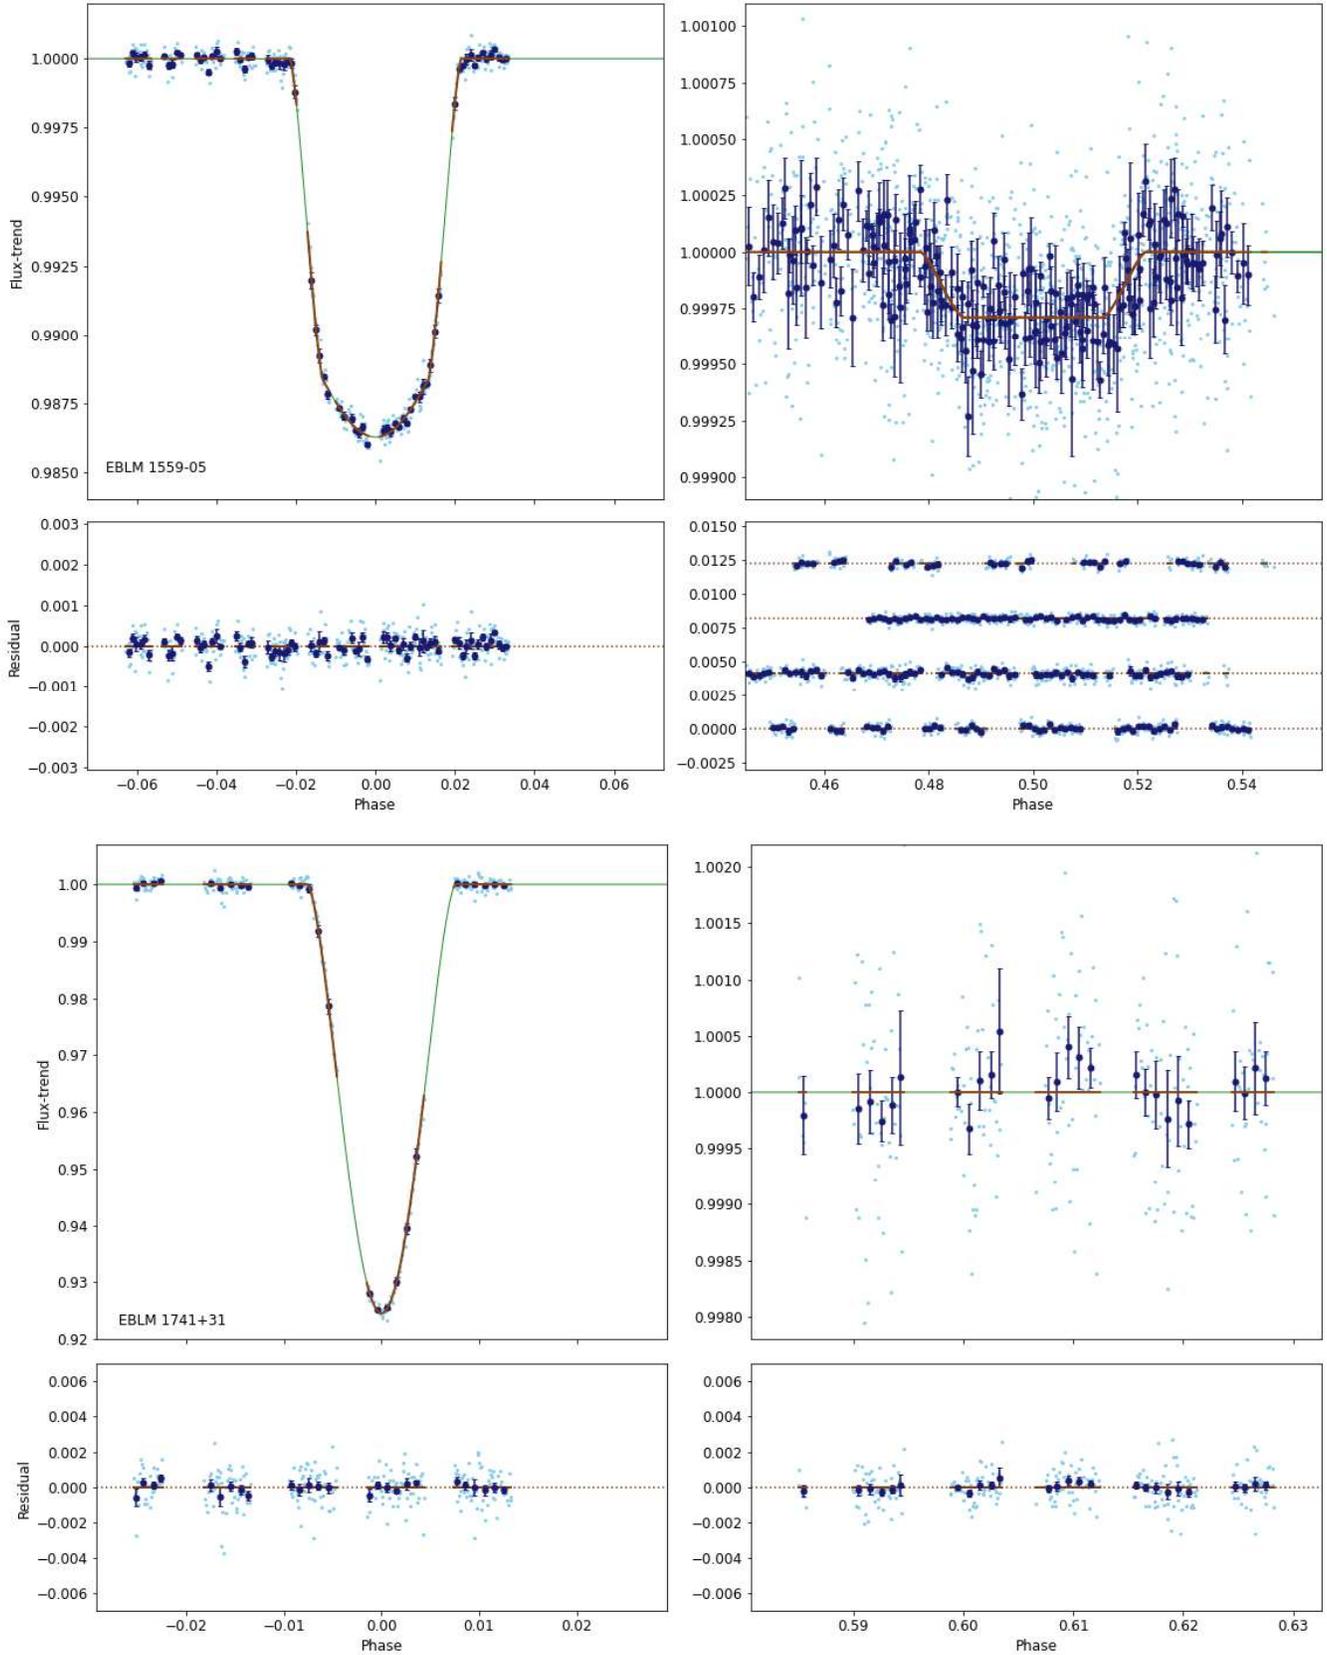

**Figure 7.** Fitted CHEOPS light curves of targets J1559-05 and J1741+31 in phase intervals around the primary and secondary eclipse events. The observed data points are shown in cyan. The transit and eclipse models are shown in green. Binned data points with error bars are shown in blue and the fit between binned data points in brown. The residual of the fit is displayed below the fitted curves.

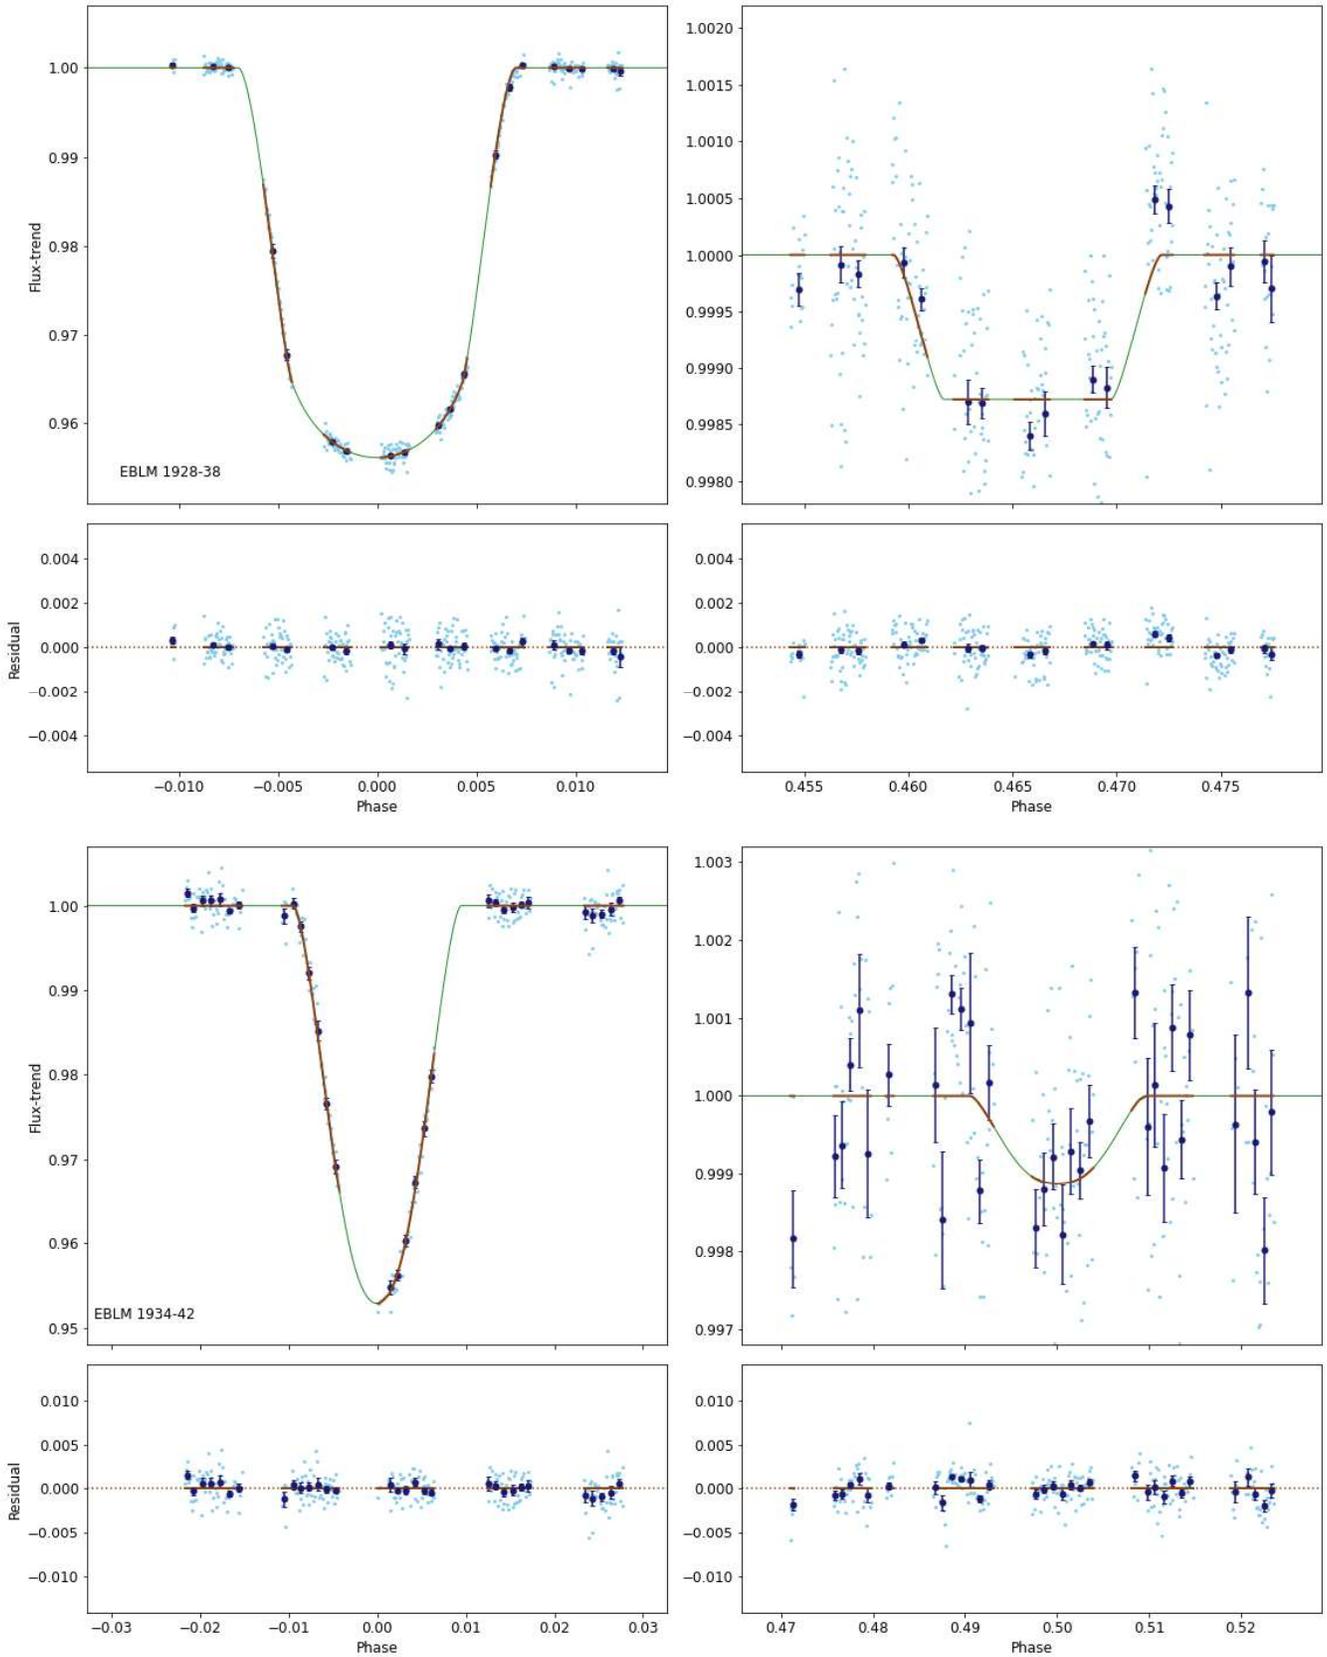

**Figure 8.** Fitted *CHEOPS* light curves of targets J1928-38 and J1934-42 in phase intervals around the primary and secondary eclipse events. The observed data points are shown in cyan. The transit and eclipse models are shown in green. Binned data points with error bars are shown in blue and the fit between binned data points in brown. The residual of the fit is displayed below the fitted curves.

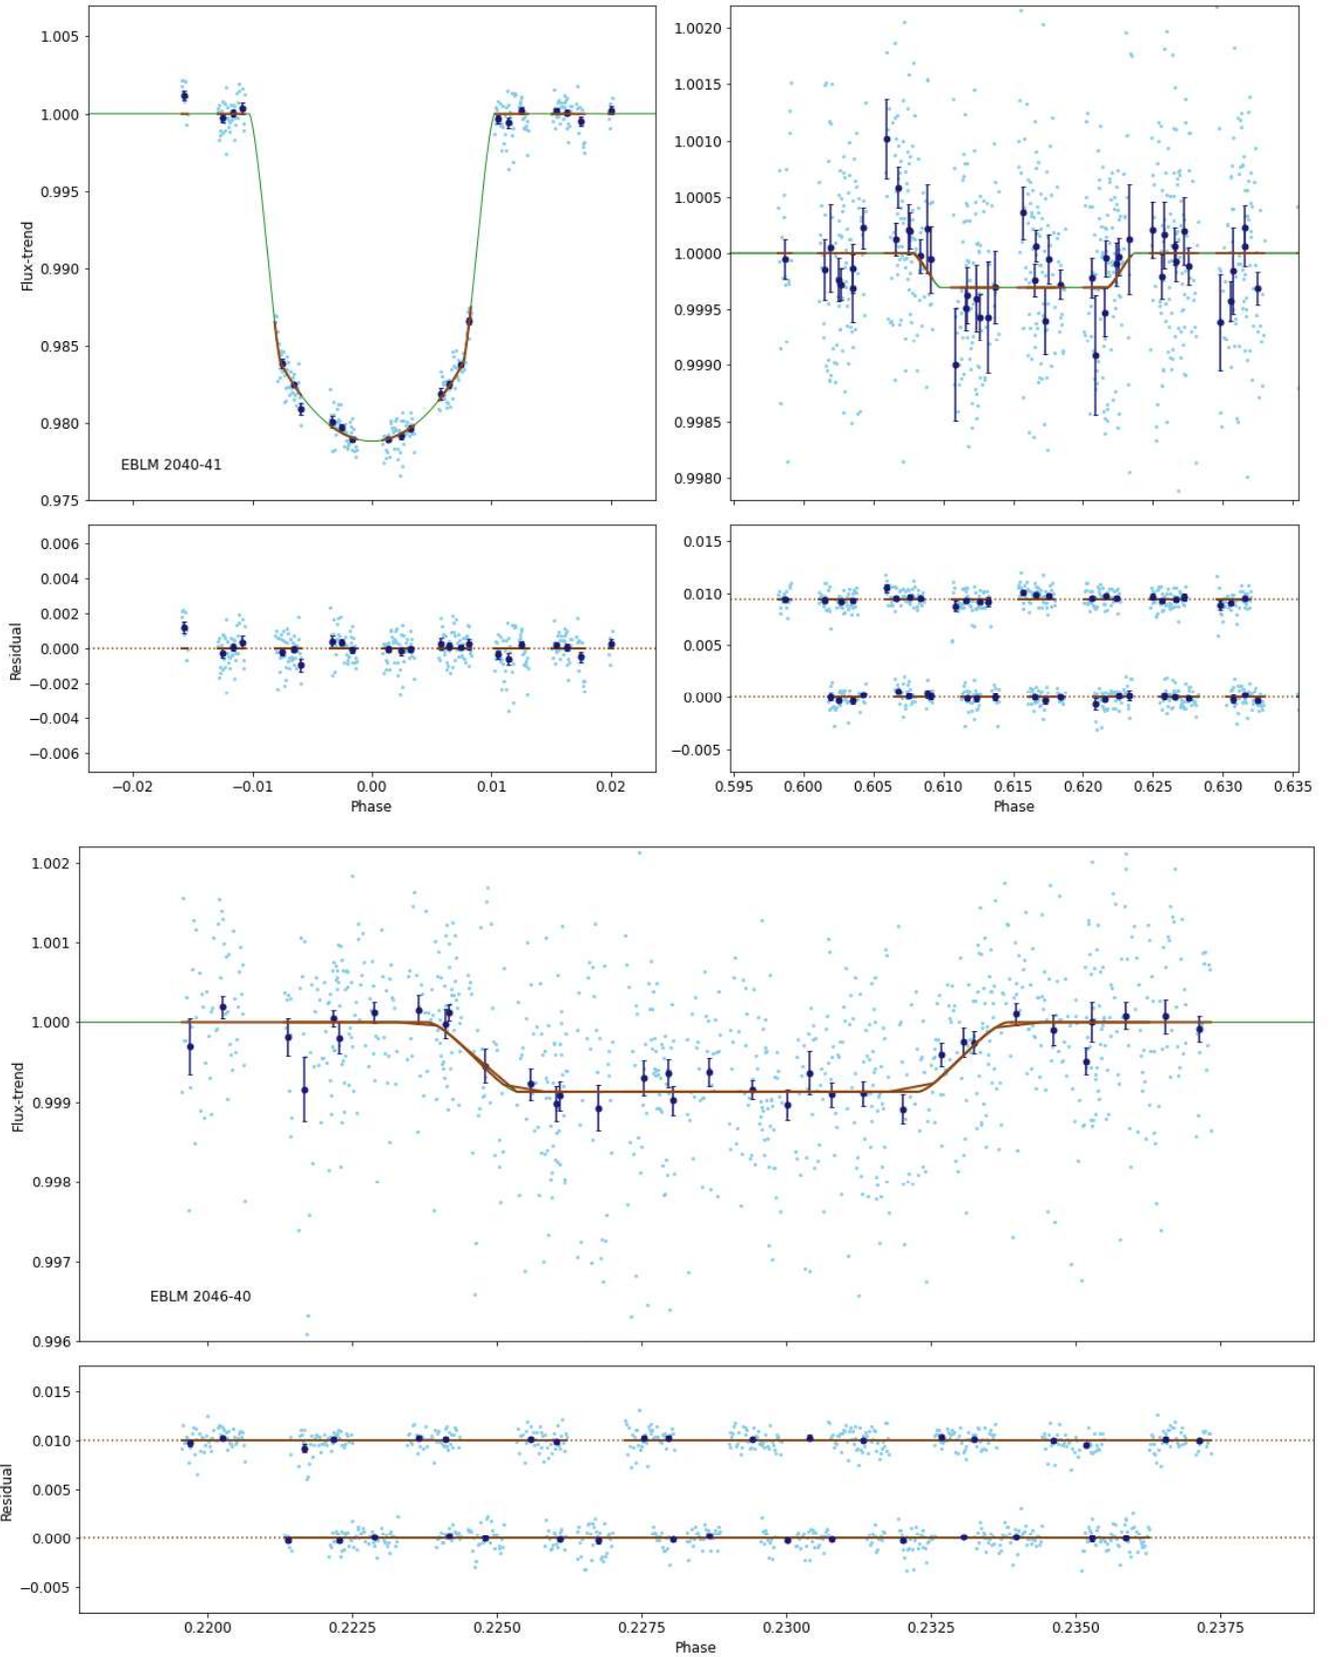

**Figure 9.** Fitted CHEOPS light curves of targets J2040-41 and J2046-40 in phase intervals around the primary and secondary eclipse events. The observed data points are shown in cyan. The transit and eclipse models are shown in green. Binned data points with error bars are shown in blue and the fit between binned data points in brown. The residual of the fit is displayed below the fitted curves.

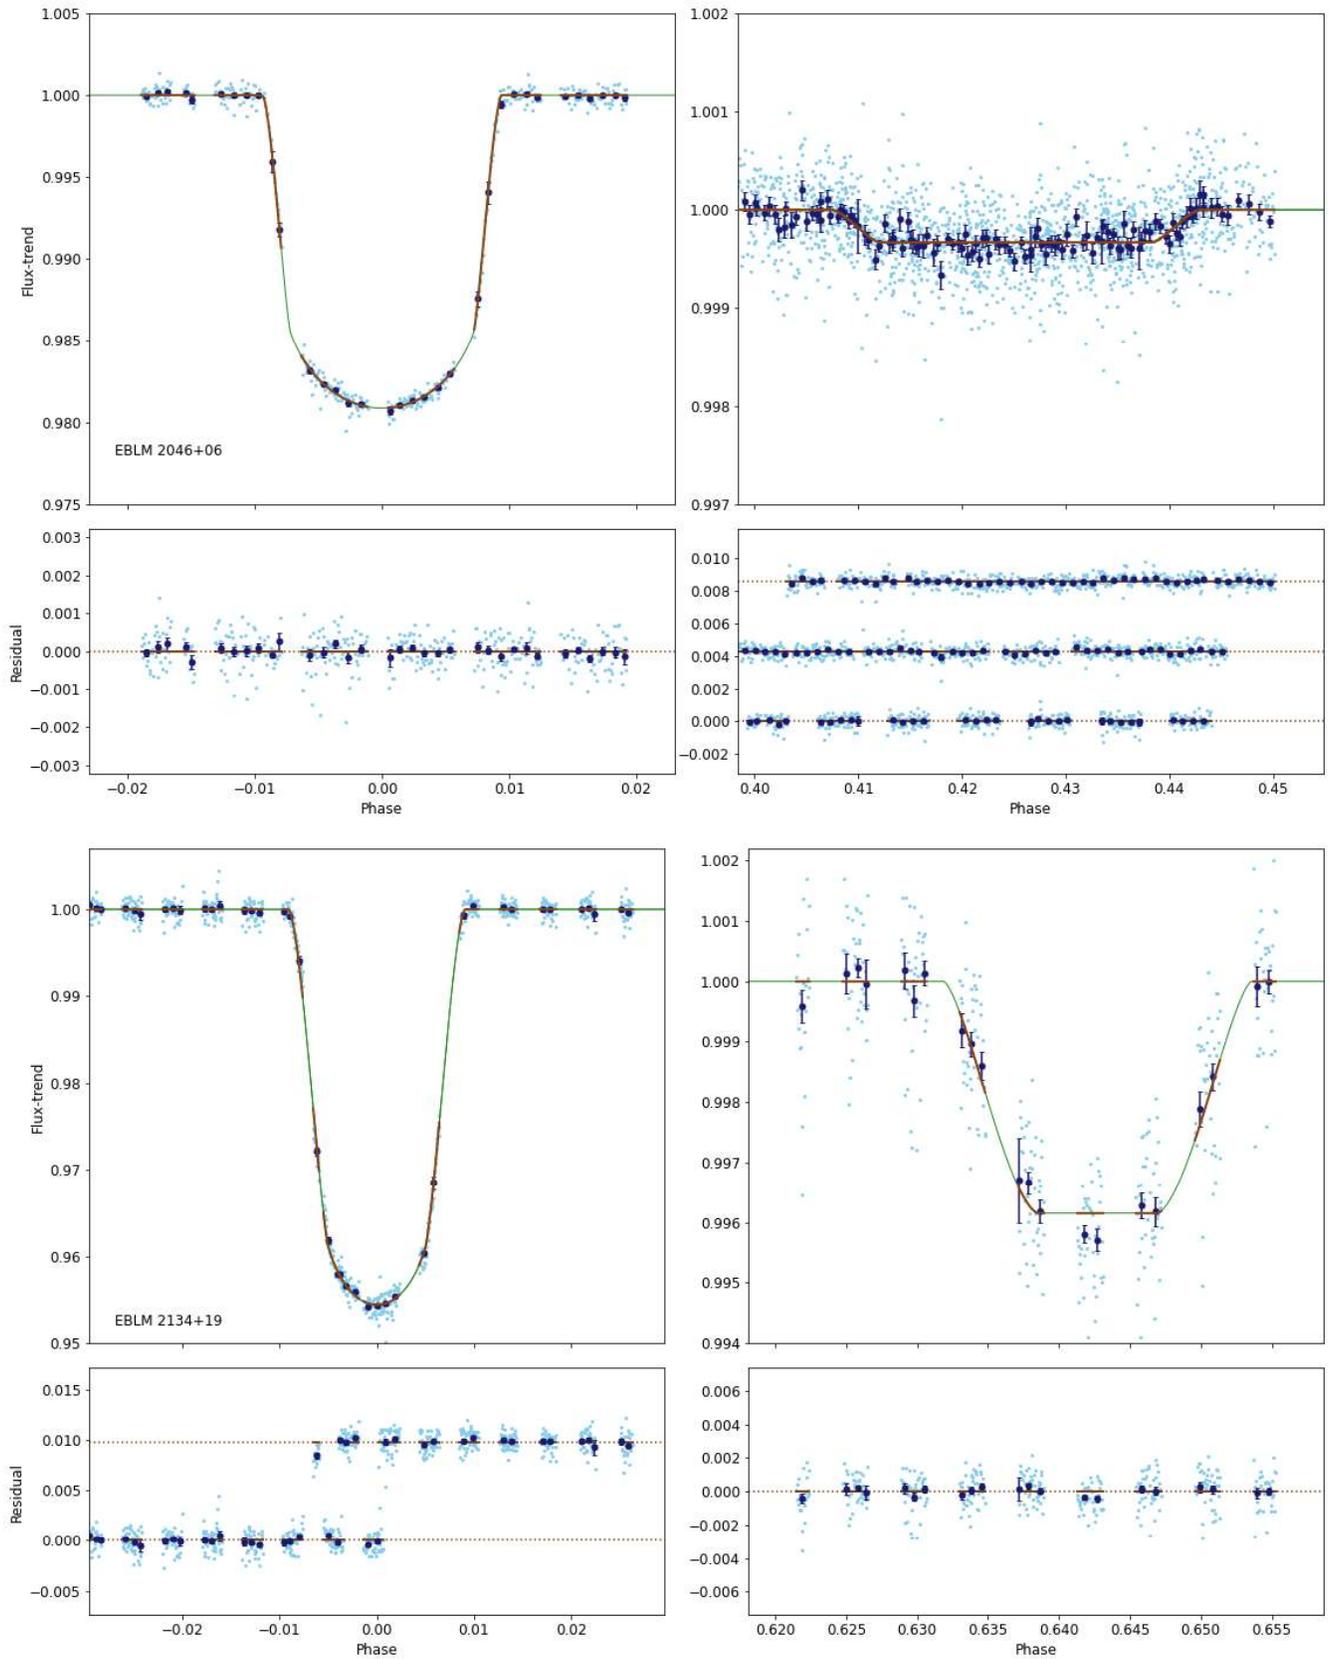

**Figure 10.** Fitted *CHEOPS* light curves of targets J2046+06 and J2134+19 in phase intervals around the primary and secondary eclipse events. The observed data points are shown in cyan. The transit and eclipse models are shown in green. Binned data points with error bars are shown in blue and the fit between binned data points in brown. The residual of the fit is displayed below the fitted curves.

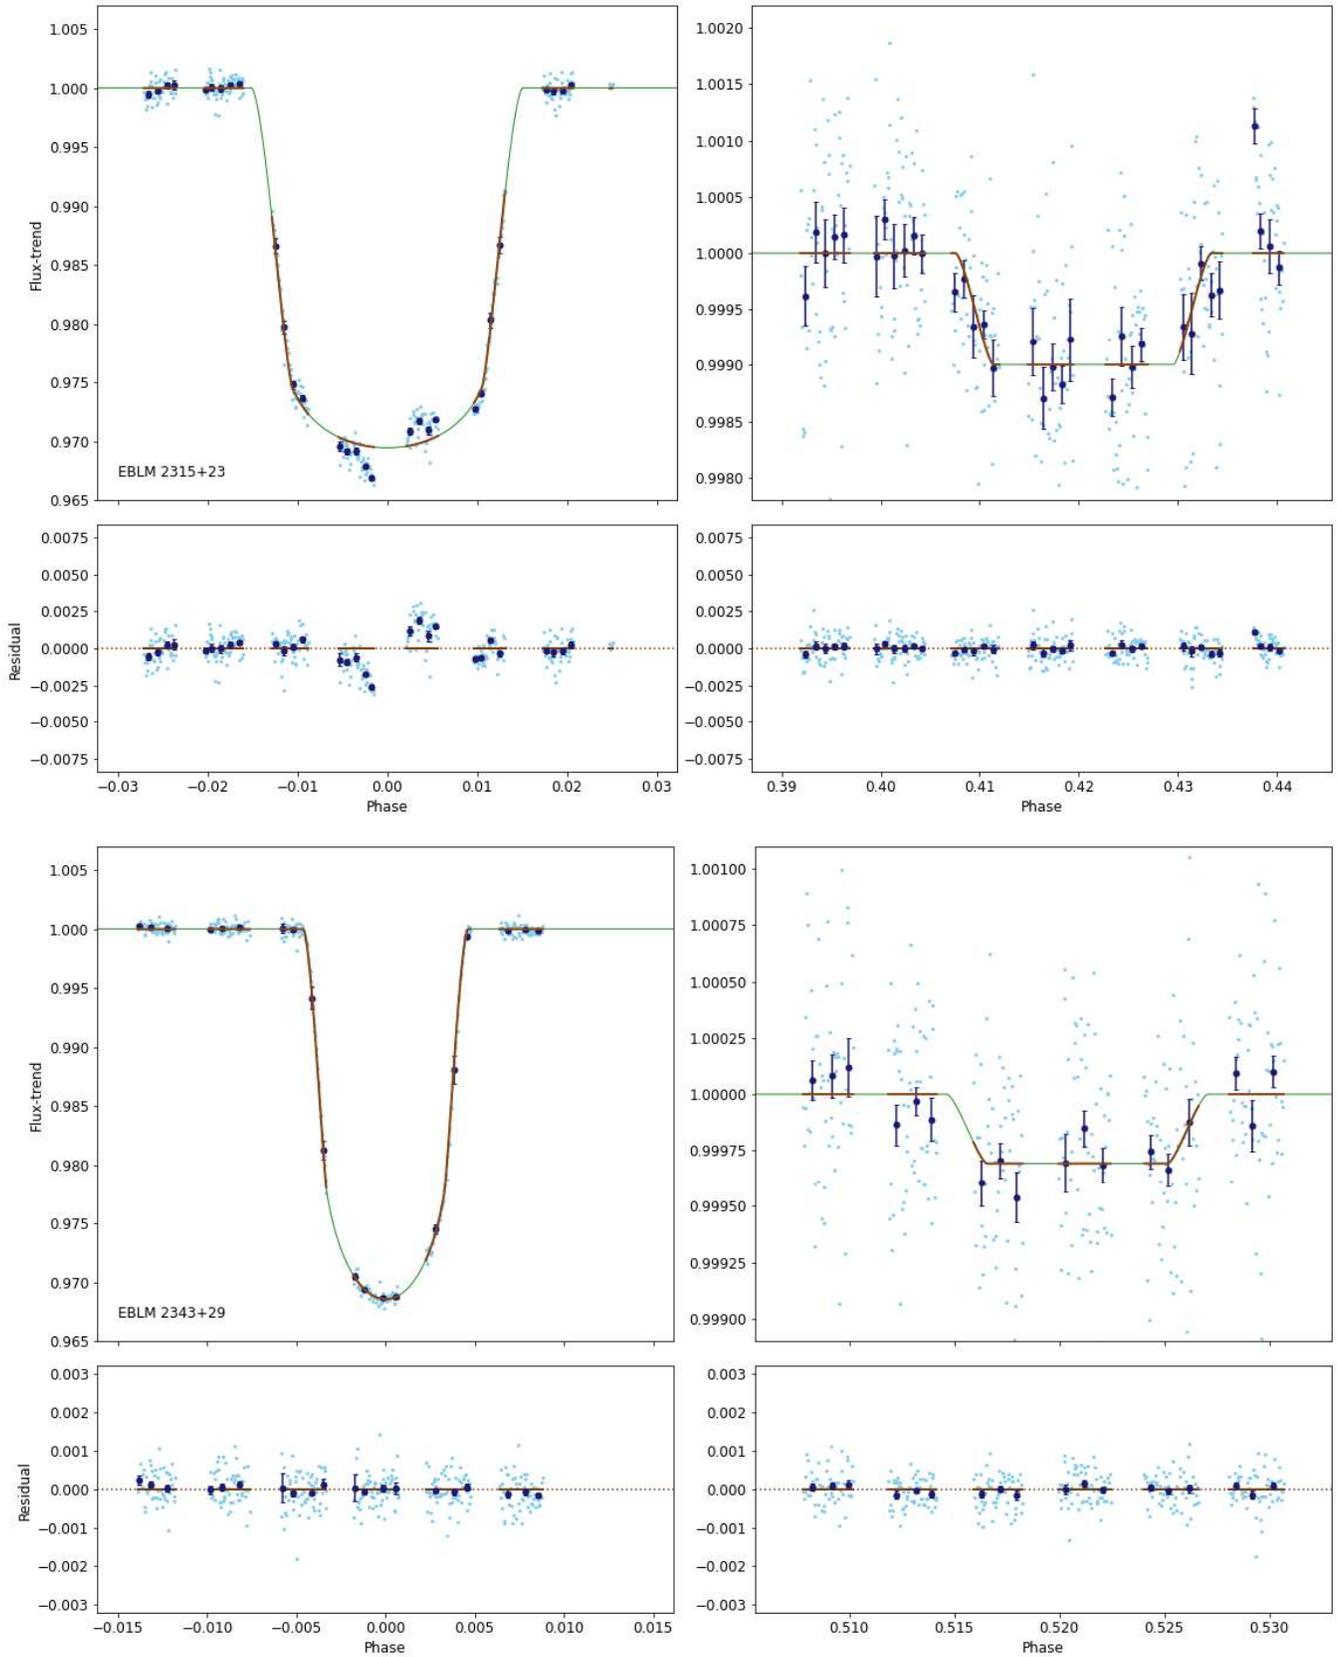

**Figure 11.** Fitted *CHEOPS* light curves of targets J2315+23 and J2343+29 in phase intervals around the primary and secondary eclipse events. The observed data points are shown in cyan. The transit and eclipse models are shown in green. Binned data points with error bars are shown in blue and the fit between binned data points in brown. The residual of the fit is displayed below the fitted curves.

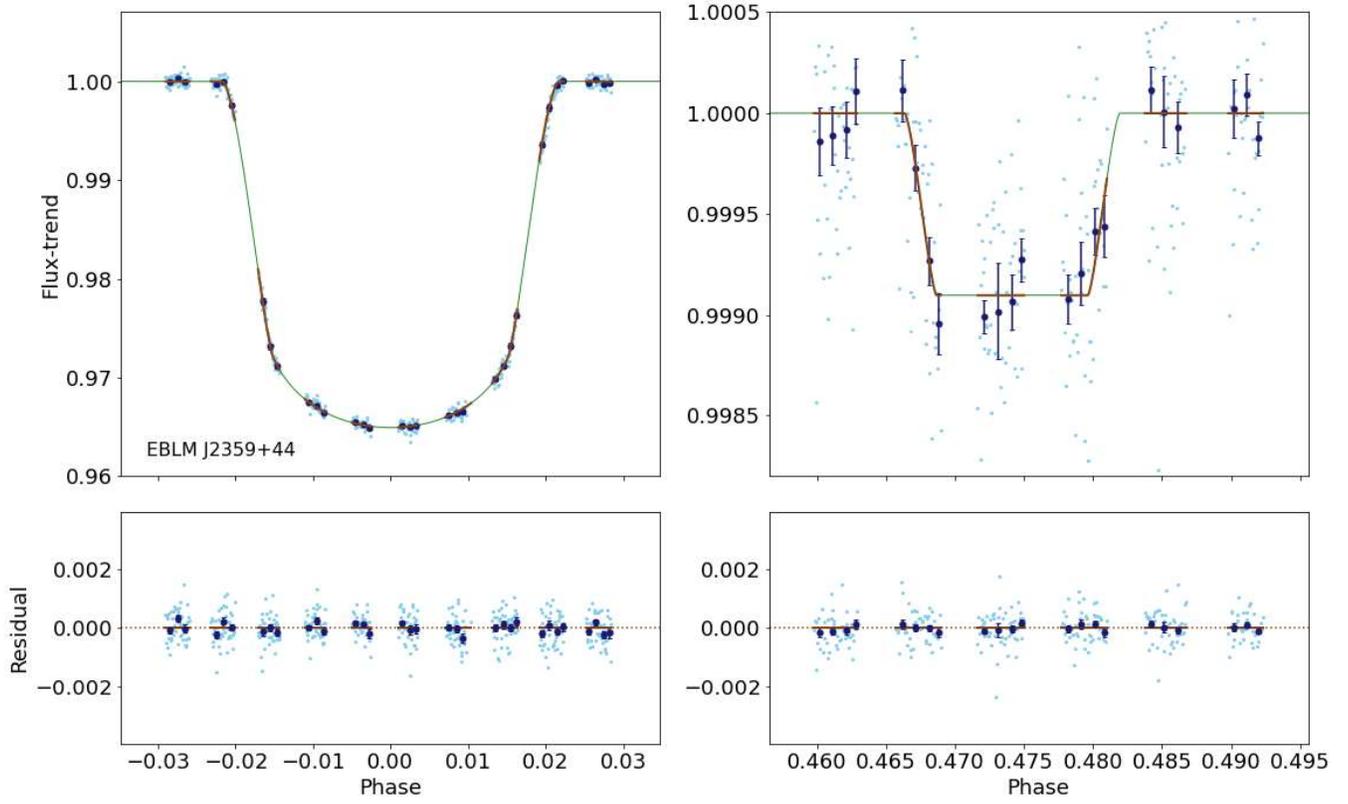

**Figure 12.** Fitted *CHEOPS* light curve of target J2359+44 in phase intervals around the primary and secondary eclipse events. The observed data points are shown in cyan. The transit and eclipse models are shown in green. Binned data points with error bars are shown in blue and the fit between binned data points in brown. The residual of the fit is displayed below the fitted curve.

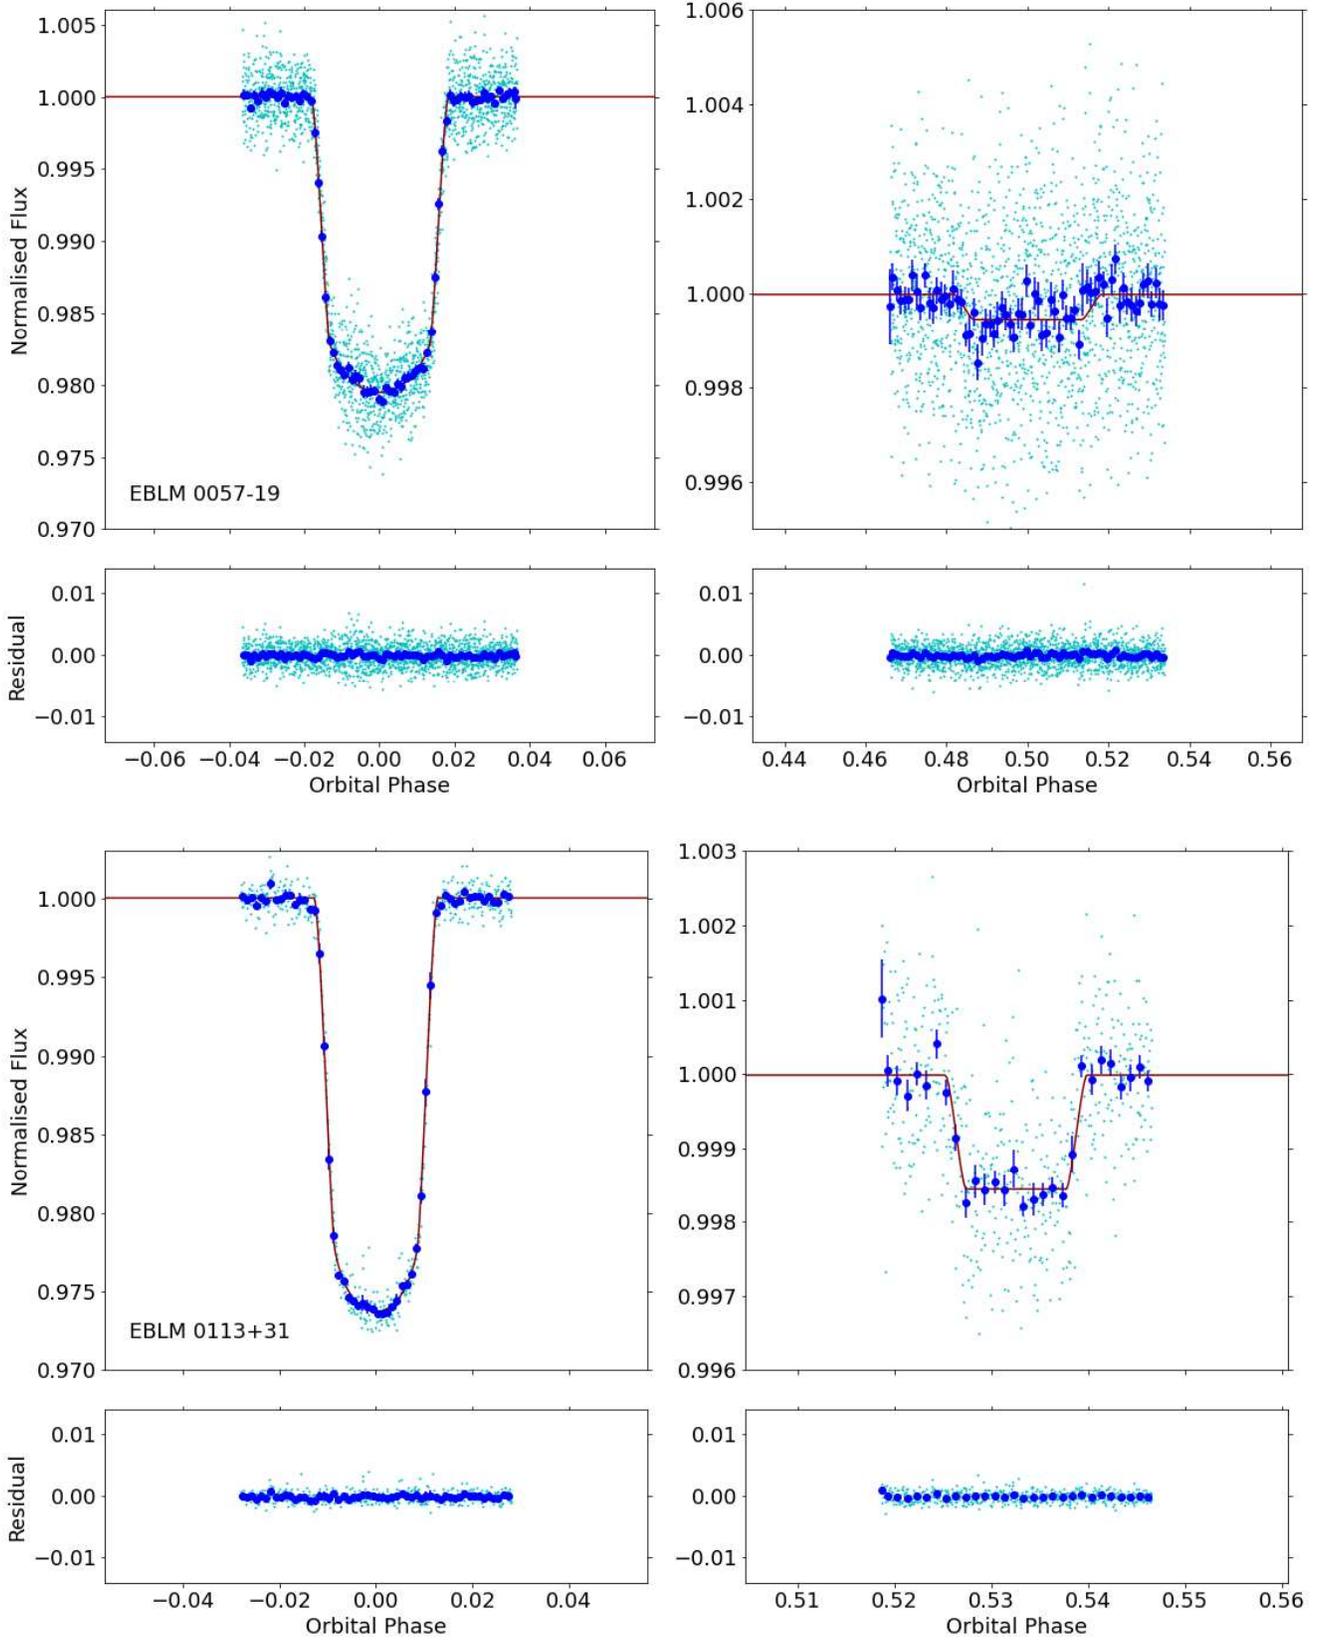

**Figure 13.** Fitted *TESS* light curves of targets J0057-19 and J0113+31 in phase intervals around the primary and secondary eclipse events. The observed data points are shown in cyan. The fitted light curve is shown in red. The residual of the fit is displayed below the fitted curves. Binned data points with error bars are shown in blue.

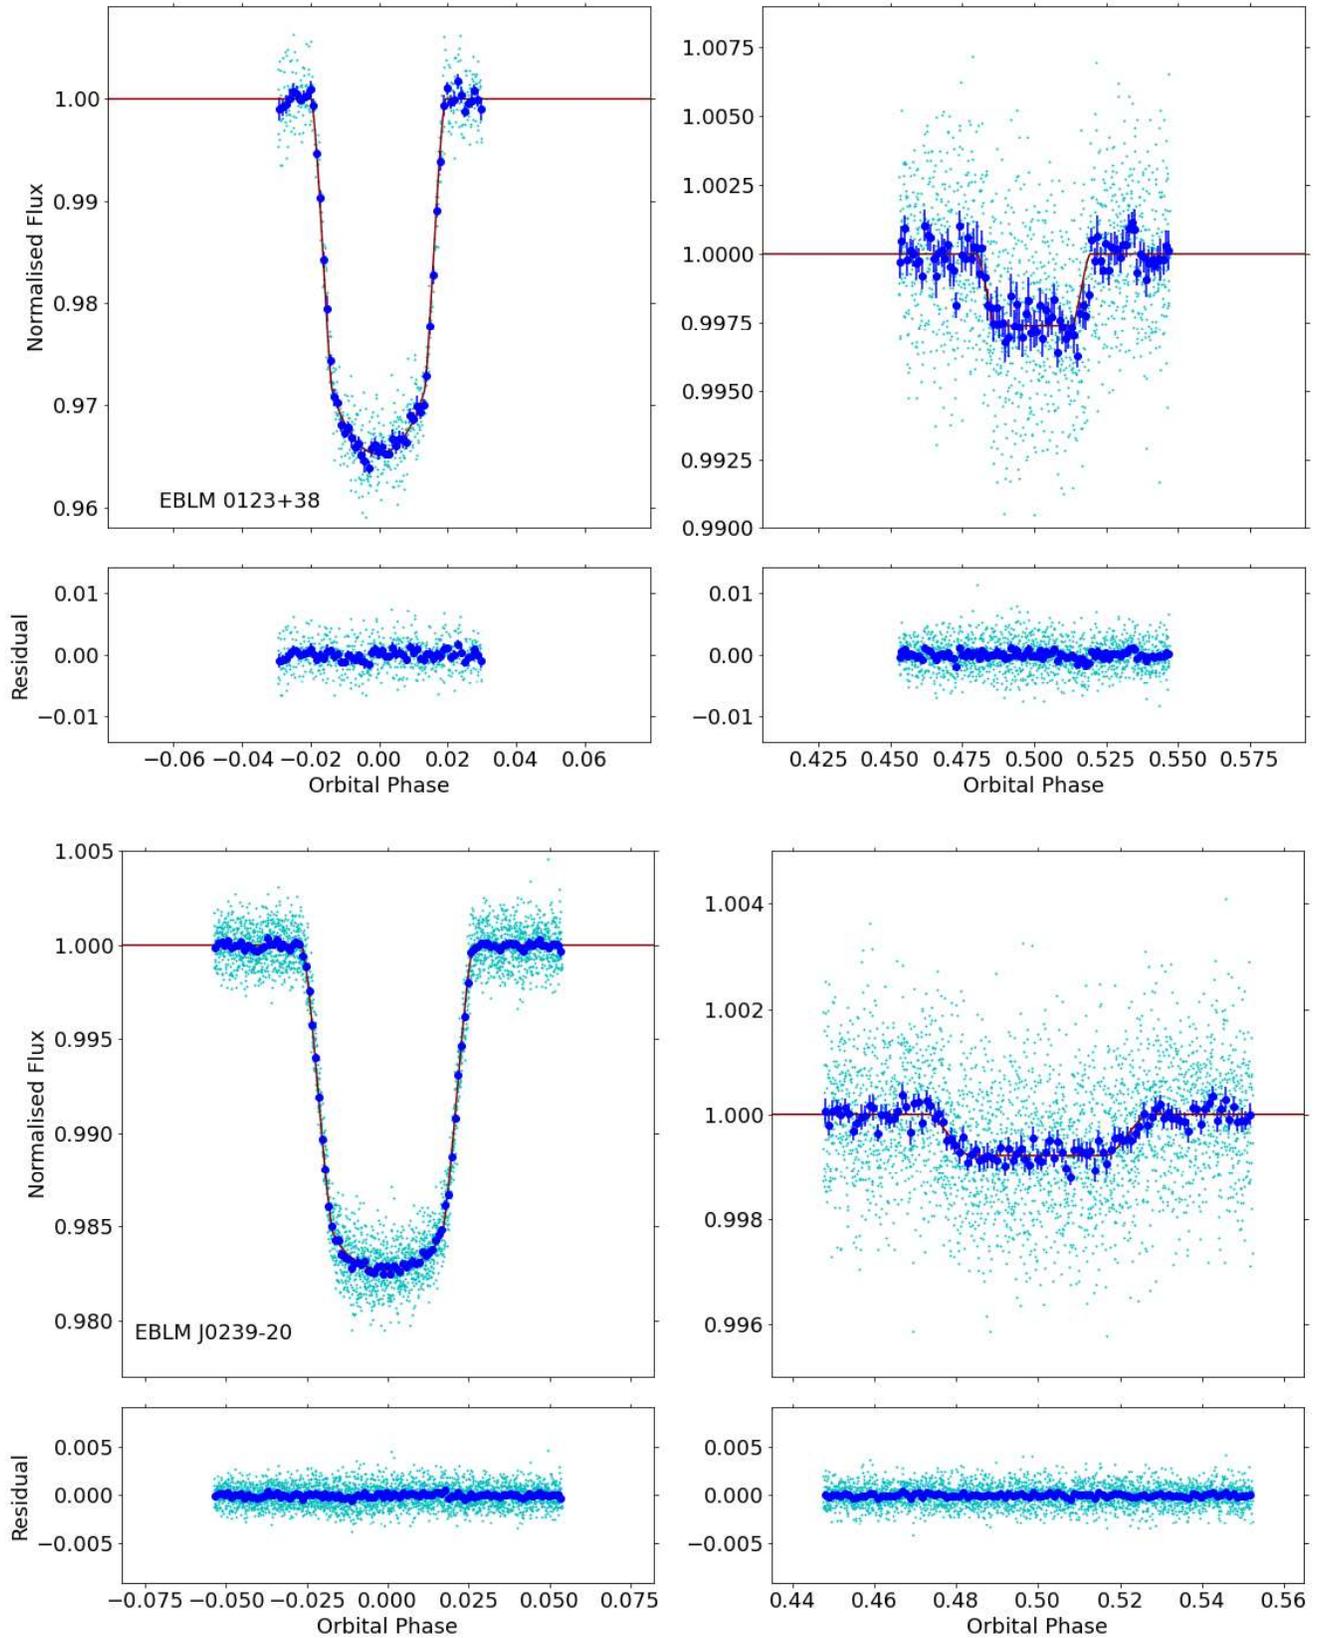

**Figure 14.** Fitted *TESS* light curves of targets J0123+38 and J0239-20 in phase intervals around the primary and secondary eclipse events. The observed data points are shown in cyan. The fitted light curve is shown in red. The residual of the fit is displayed below the fitted curves. Binned data points with error bars are shown in blue.

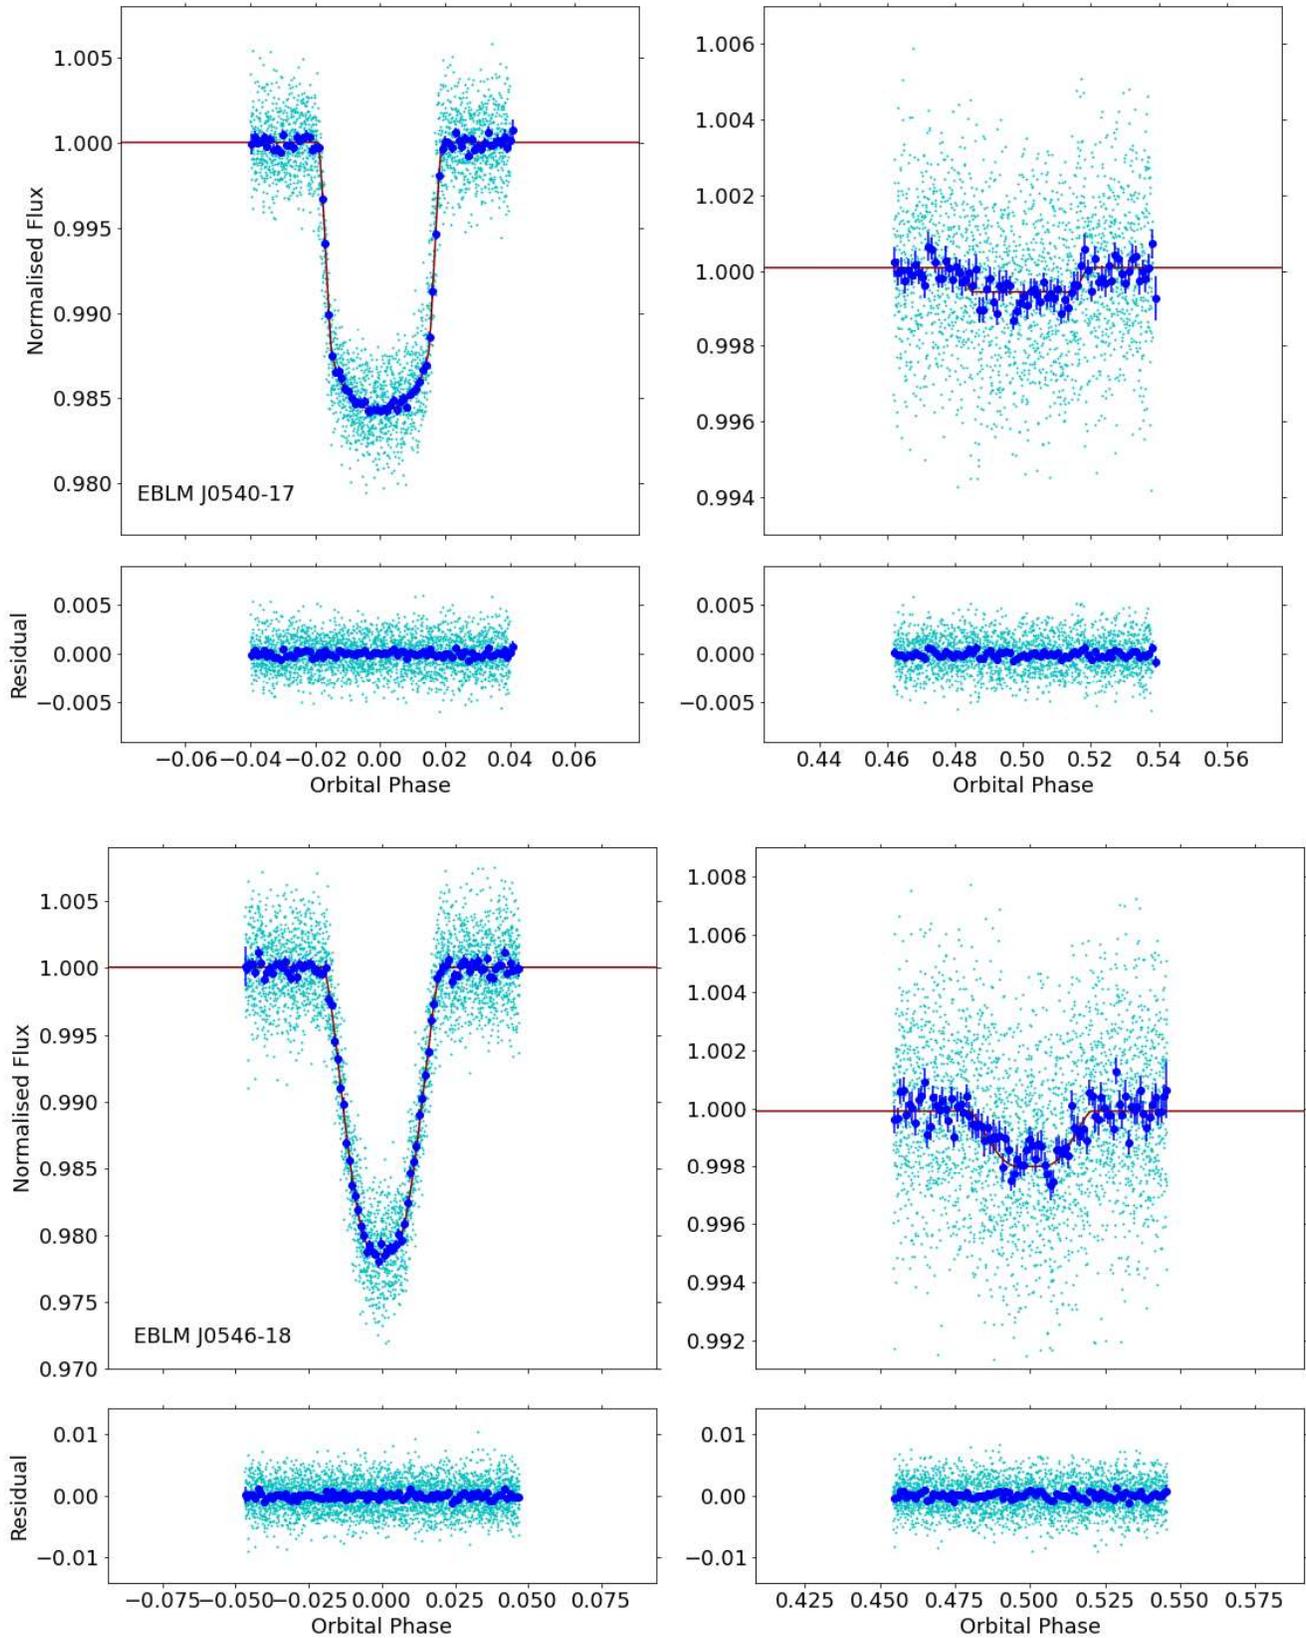

**Figure 15.** Fitted TESS light curves of targets J0540-17 and J0546-18 in phase intervals around the primary and secondary eclipse events. The observed data points are shown in cyan. The fitted light curve is shown in red. The residual of the fit is displayed below the fitted curves. Binned data points with error bars are shown in blue.

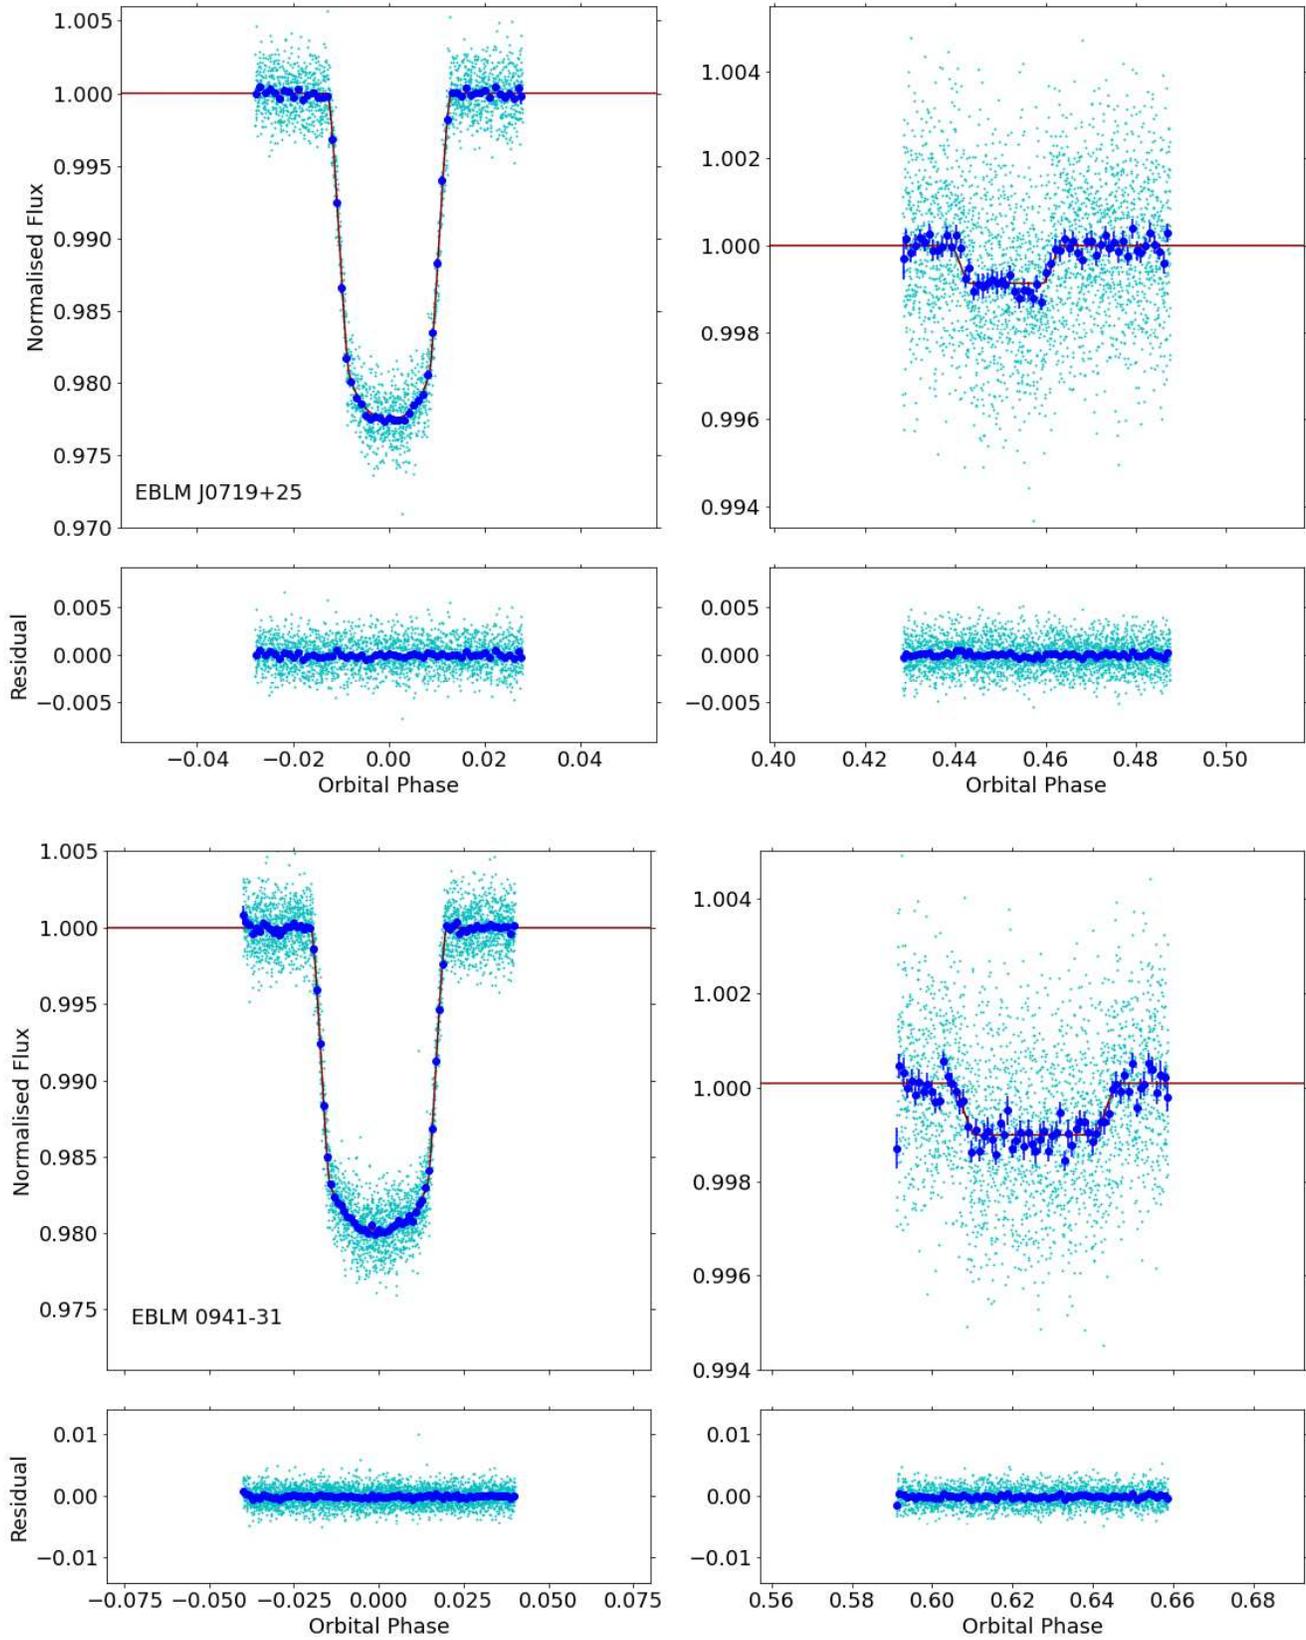

**Figure 16.** Fitted *TESS* light curves of targets J0719+25 and J0941-31 in phase intervals around the primary and secondary eclipse events. The observed data points are shown in cyan. The fitted light curve is shown in red. The residual of the fit is displayed below the fitted curves. Binned data points with error bars are shown in blue.

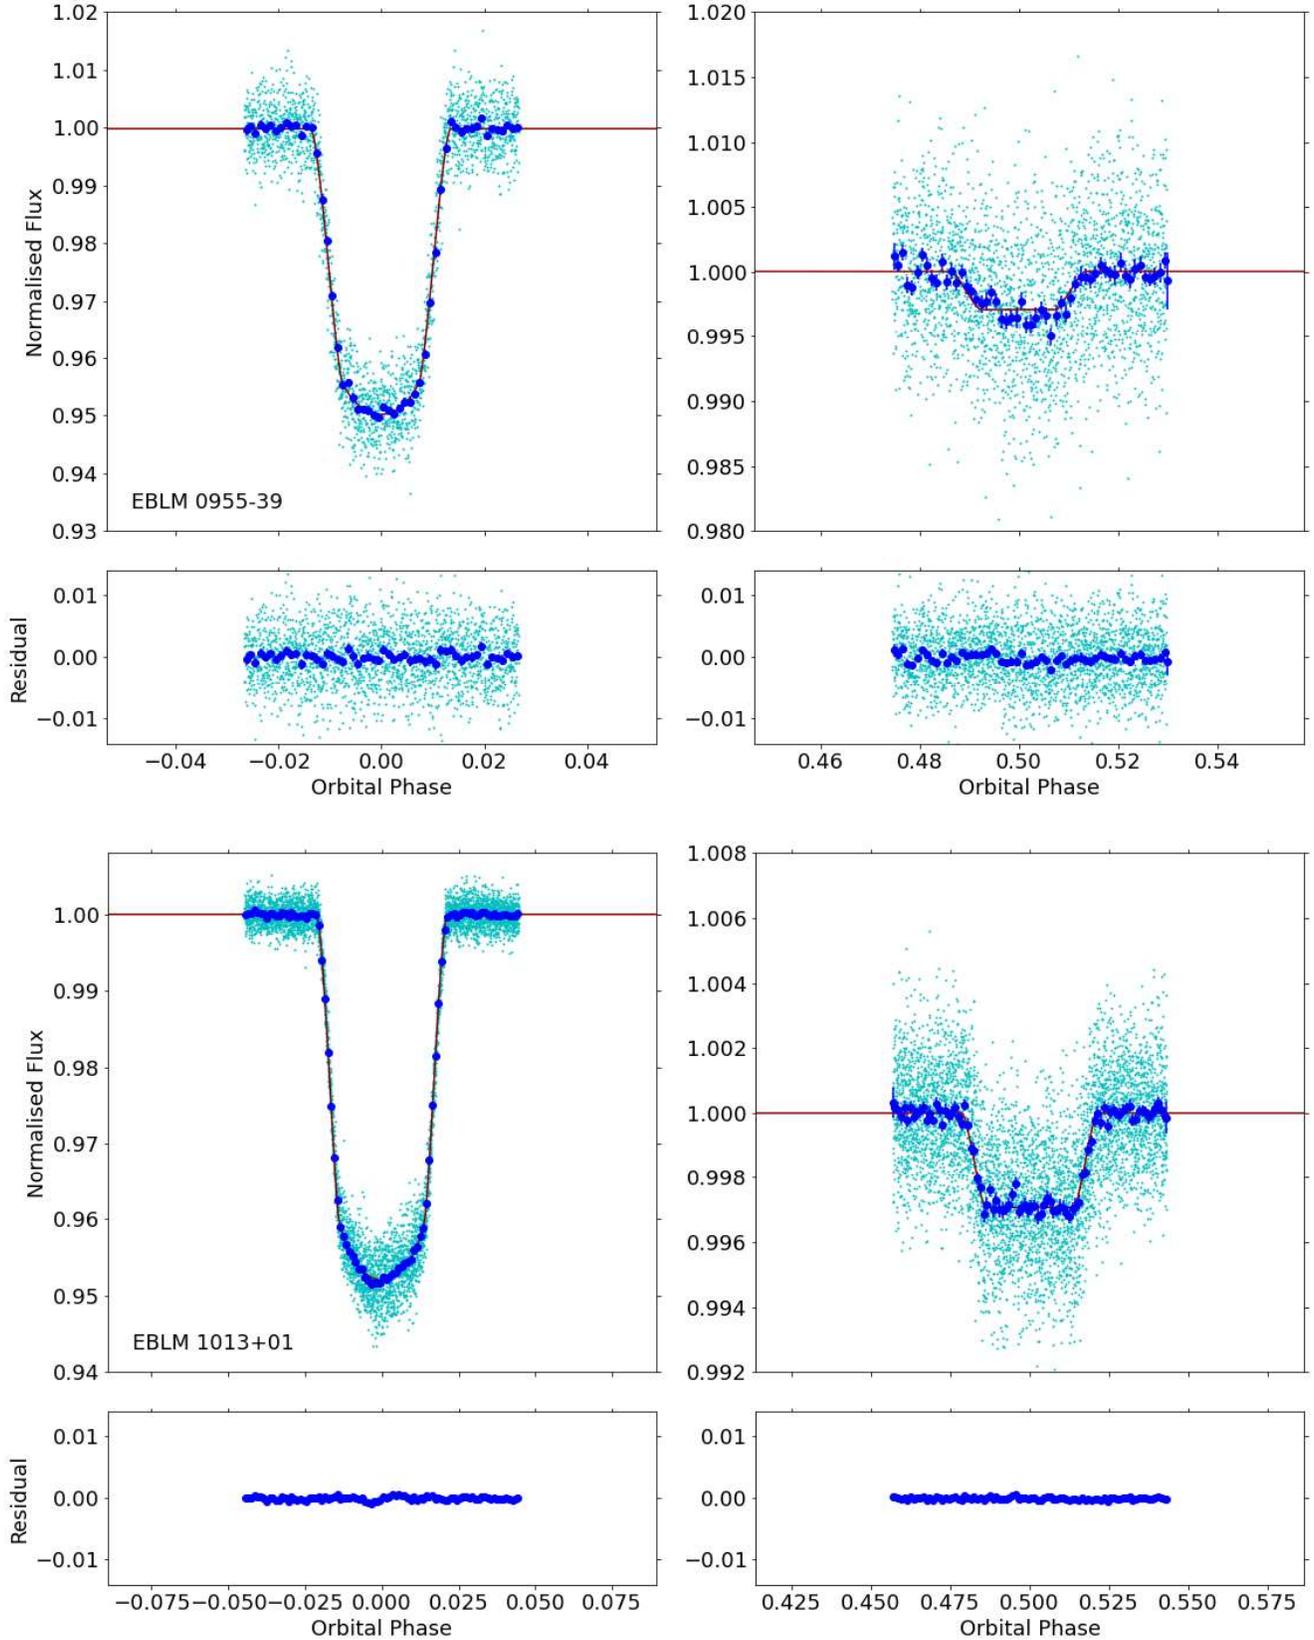

**Figure 17.** Fitted *TESS* light curves of targets J0955-39 and J1013+01 in phase intervals around the primary and secondary eclipse events. The observed data points are shown in cyan. The fitted light curve is shown in red. The residual of the fit is displayed below the fitted curves. Binned data points with error bars are shown in blue.

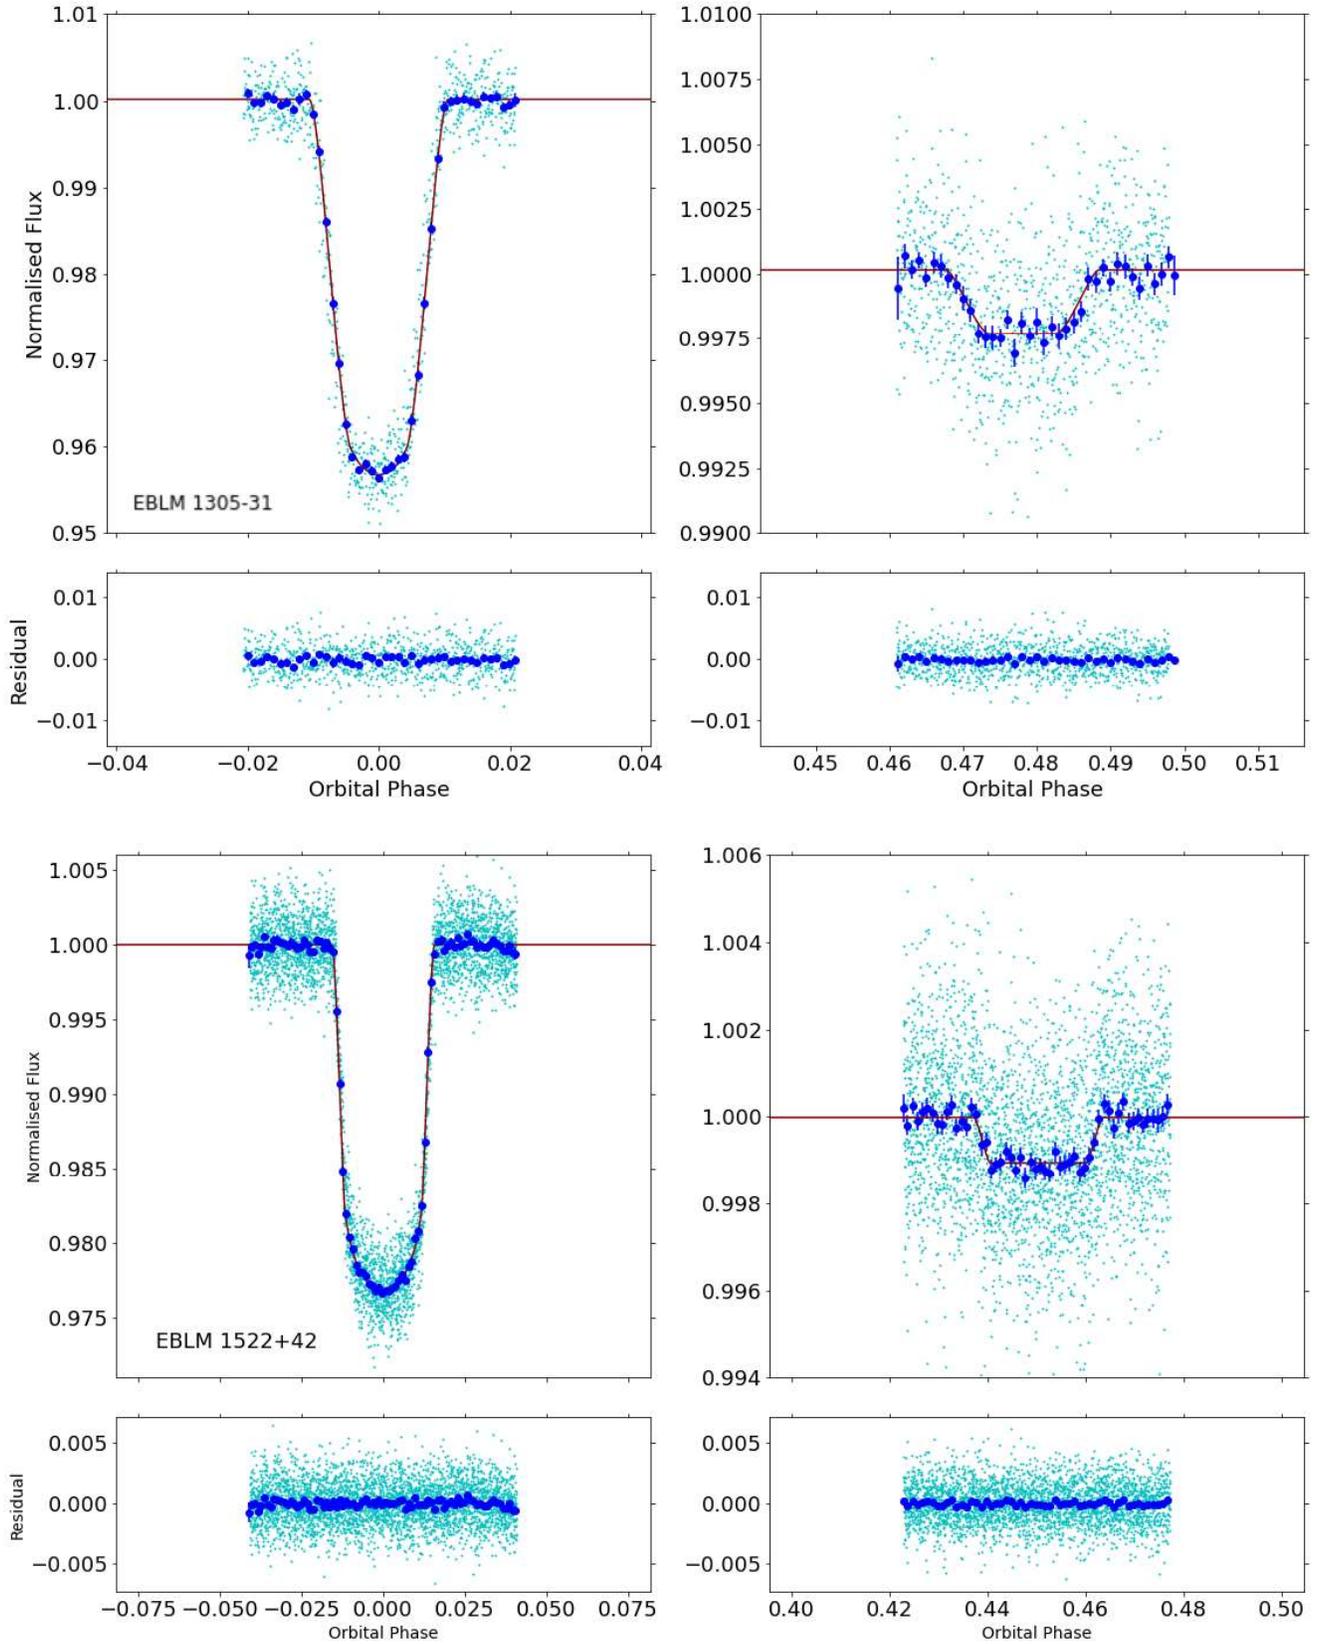

**Figure 18.** Fitted *TESS* light curves of targets J1305-31 and J1522+42 in phase intervals around the primary and secondary eclipse events. The observed data points are shown in cyan. The fitted light curve is shown in red. The residual of the fit is displayed below the fitted curves. Binned data points with error bars are shown in blue.

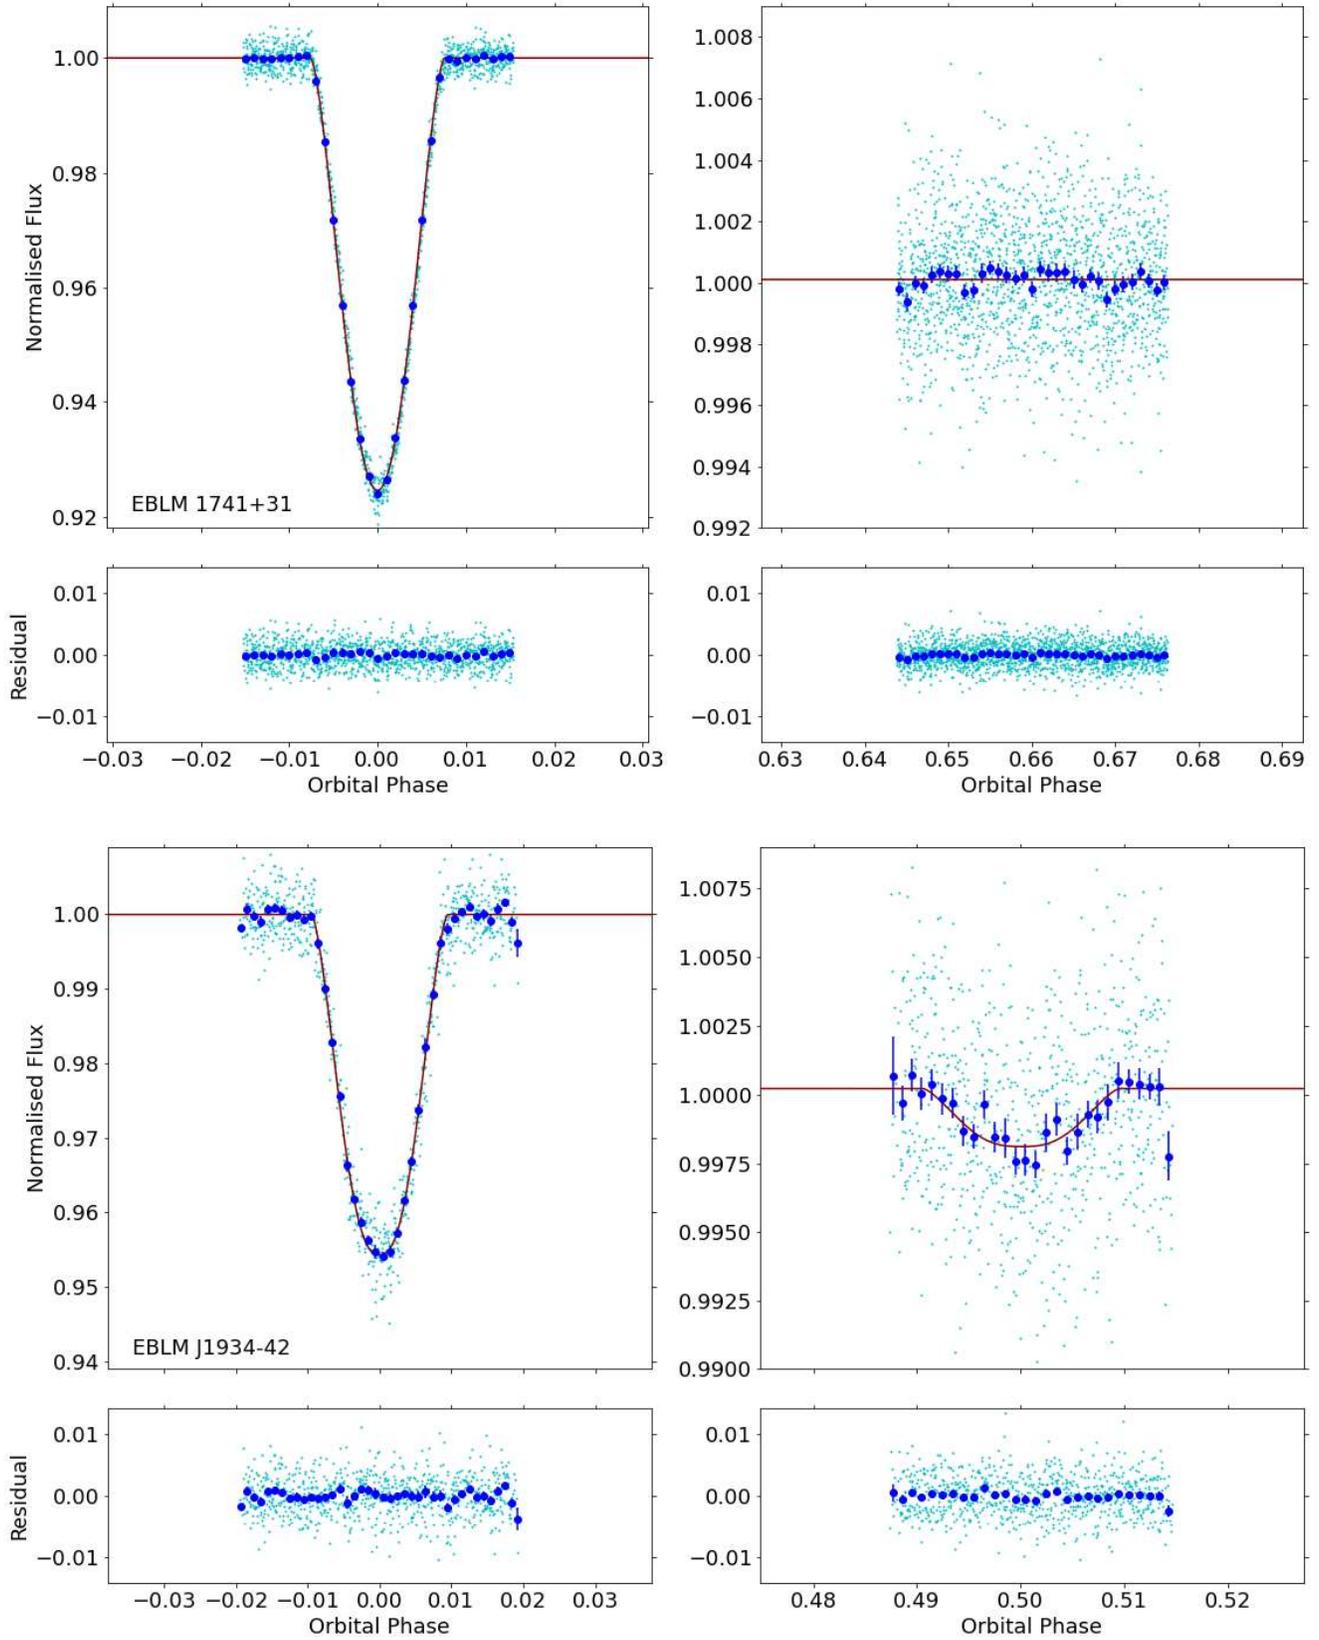

**Figure 19.** Fitted *TESS* light curves of targets J1741+31 and J1934-42 in phase intervals around the primary and secondary eclipse events. The observed data points are shown in cyan. The fitted light curve is shown in red. The residual of the fit is displayed below the fitted curves. Binned data points with error bars are shown in blue.

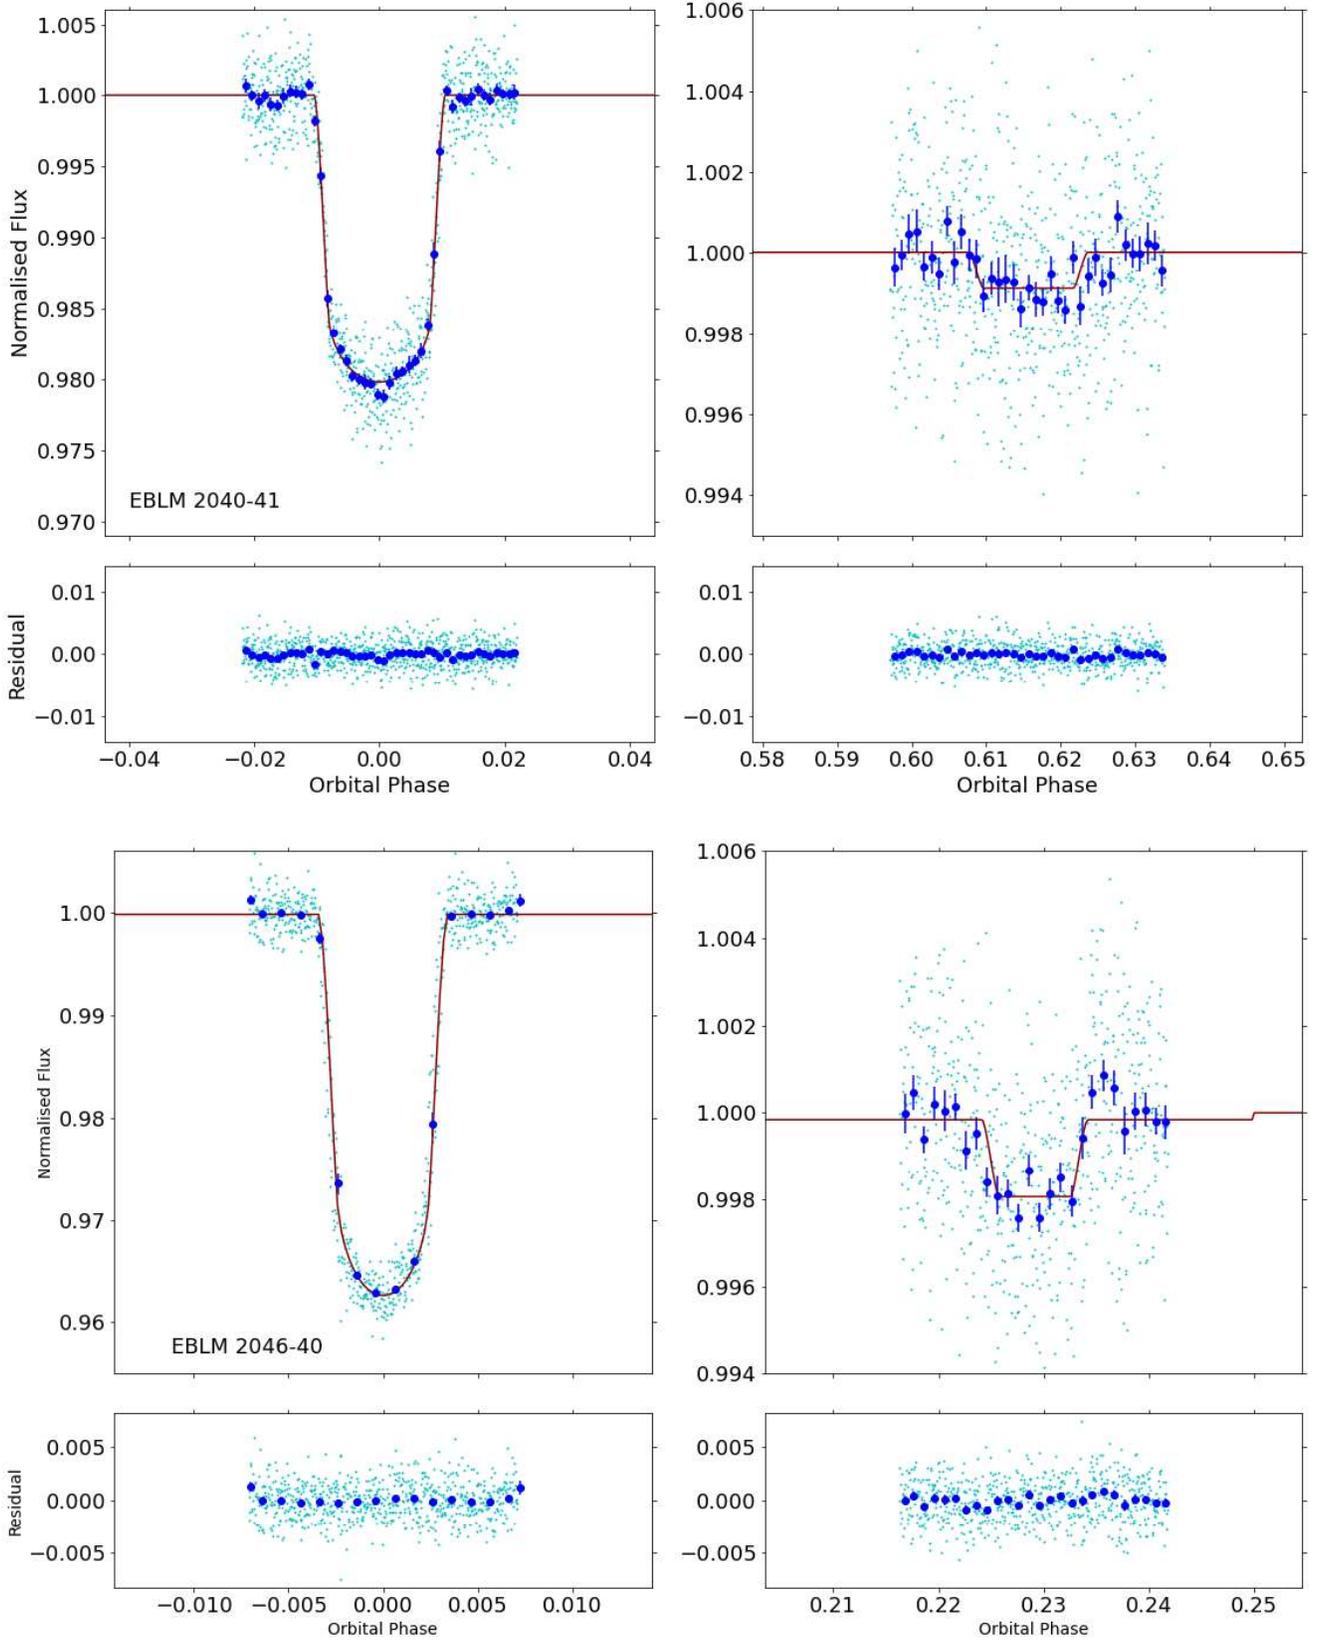

**Figure 20.** Fitted *TESS* light curves of targets J2040-41 and J2046-40 in phase intervals around the primary and secondary eclipse events. The observed data points are shown in cyan. The fitted light curve is shown in red. The residual of the fit is displayed below the fitted curves. Binned data points with error bars are shown in blue.

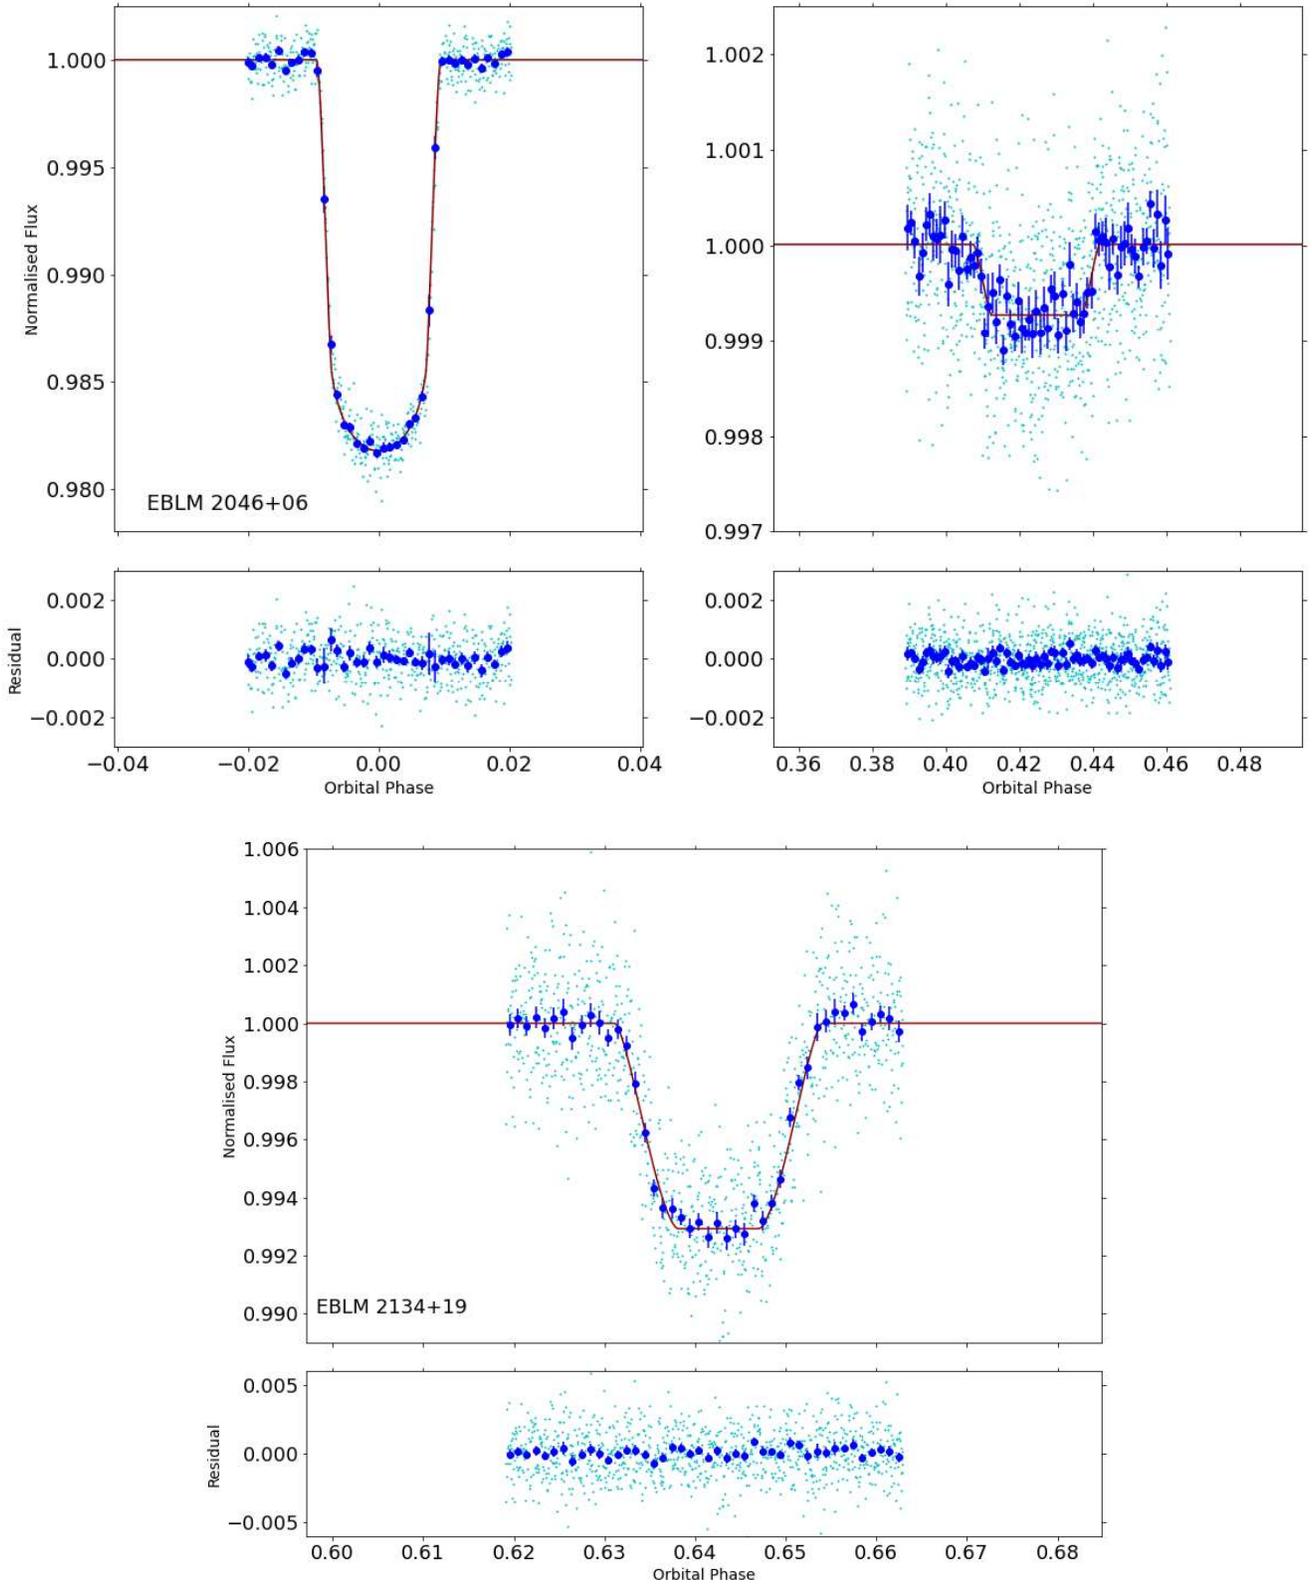

**Figure 21.** Fitted *TESS* light curves of targets J2046+06 and J2134+19 in phase intervals around the primary and secondary eclipse events. The observed data points are shown in cyan. The fitted light curve is shown in red. The residual of the fit is displayed below the fitted curves. Binned data points with error bars are shown in blue.

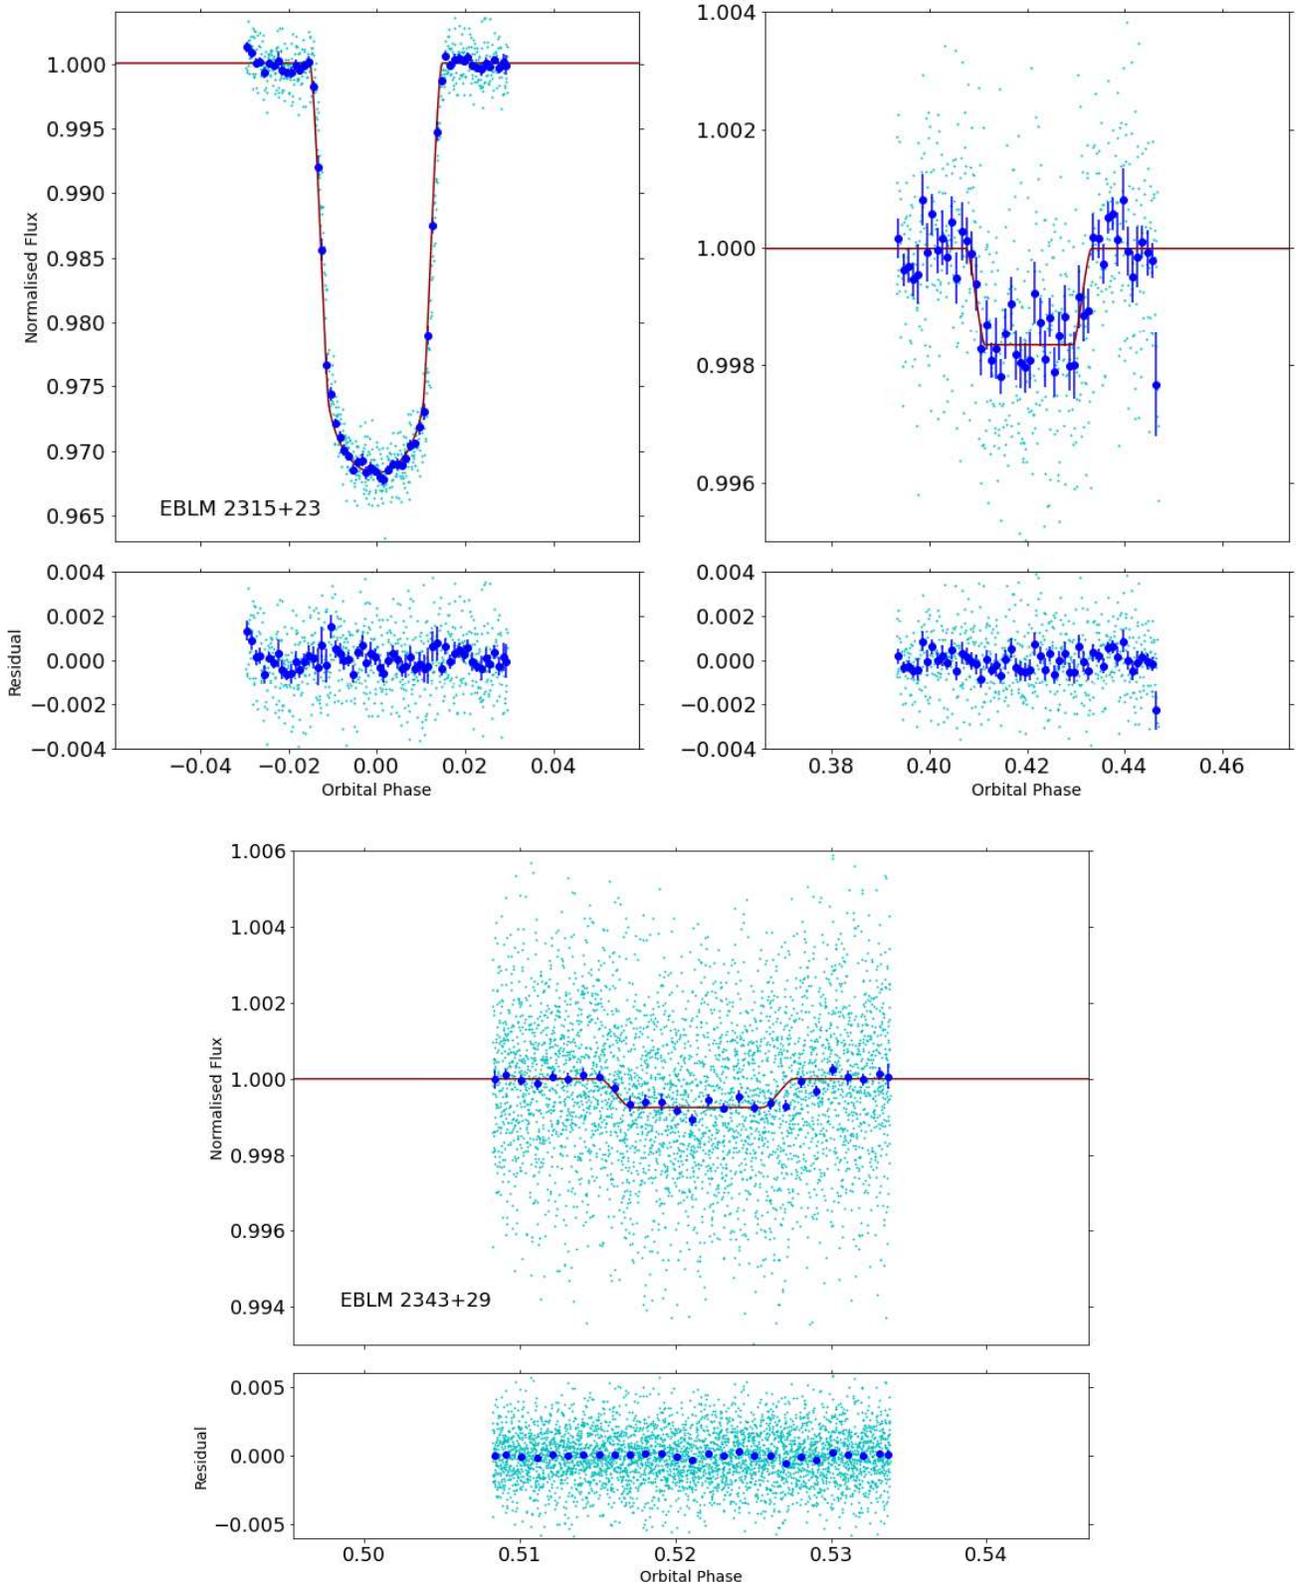

**Figure 22.** Fitted *TESS* light curves of targets J2315+23 and J2343+29 in phase intervals around the primary and secondary eclipse events. The observed data points are shown in cyan. The fitted light curve is shown in red. The residual of the fit is displayed below the fitted curves. Binned data points with error bars are shown in blue.

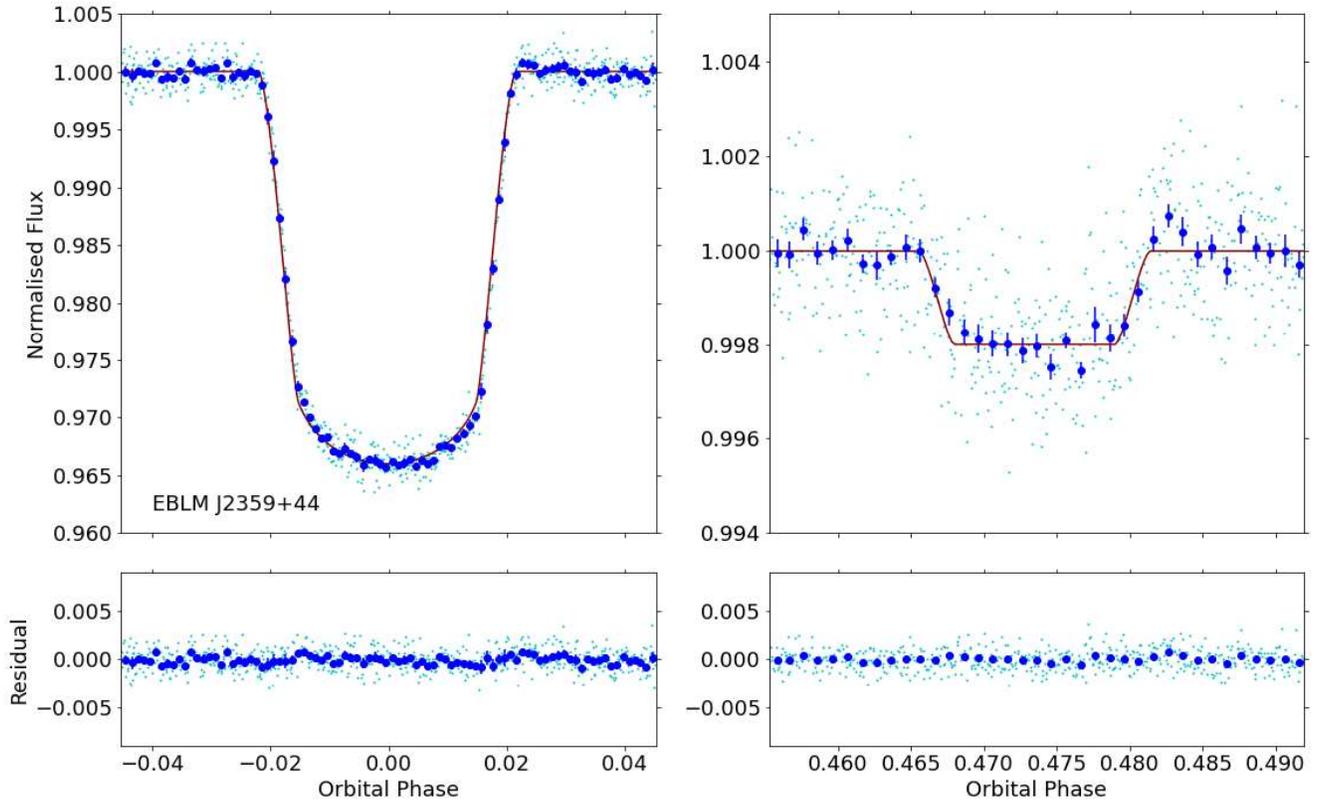

**Figure 23.** Fitted *TESS* light curve of the target J2359+44 in phase intervals around the primary and secondary eclipse events. The observed data points are shown in cyan. The fitted light curve is shown in red. The residual of the fit is displayed below the fitted curves. Binned data points with error bars are shown in blue.

This paper has been typeset from a  $\text{\TeX/L\AA\TeX}$  file prepared by the author.
